# Supplementary material for: Identifying Neutron Sources using Recoil and Time-of-Flight Spectroscopy
Source: arXiv:2512.10044 ancillary file (2026-03-16)
Supplement: Supplementary file 1 [file supplementary_materials.pdf]

# Supplementary Information for

## Identifying Neutron Sources using Recoil and Time-of-Flight Spectroscopy

David Breitenmoser[1,*], Ricardo Lopez[1], Shaun D. Clarke[1], Sara A. Pozzi[1]

[1]Department of Nuclear Engineering & Radiological Sciences, University of Michigan, 2355 Bonisteel Blvd., Ann Arbor, MI 48109-2104, United States of America

[*]Lead and contact author: David Breitenmoser (E-Mail: dbreiten@umich.edu, ORCID: 0000-0003-0339-6592)

**The PDF includes:**

Supplementary Methods S1.1–S1.3
Supplementary Figures S1–S22
Supplementary Table S1
Supplementary References

# Contents

**List of Supplementary Figures** SIII

**List of Supplementary Tables** SIV

**S1 Supplementary Methods** S1

S1.1 Neutron Spectroscopy Experiments . . . . . S1

S1.1.1 Experimental Setup . . . . . S1

S1.1.2 Neutron Spectrometer . . . . . S1

S1.1.3 Data Reduction . . . . . S3

S1.1.4 Background Evaluation . . . . . S4

S1.2 Template Bank Generation . . . . . S6

S1.2.1 Generalized Additive Machine Learning Model . . . . . S6

S1.2.2 Template Bias Assessment . . . . . S6

S1.3 Bayesian Computations . . . . . S13

S1.3.1 Bayesian Inference Pipeline . . . . . S13

S1.3.2 Event Scaling . . . . . S21

**Supplementary References** S31

# List of Supplementary Figures


S1 Experimental setup . . . S2
S2 Background quantification . . . S5
S3 Generalized additive model templates . . . S7
S4 Template bias quantification . . . S8
S5 Bayesian evidence results using recoil spectroscopy (10 keV reduced spectral band) . . . S9
S6 Bayesian evidence results using recoil spectroscopy (10 keV increased spectral band) . . S10
S7 Bayesian evidence results using TOF spectroscopy (10 keV reduced spectral band) . . . . S11
S8 Bayesian evidence results using TOF spectroscopy (10 keV increased spectral band) . . . S12
S9 Posterior distribution for recoil spectroscopy experiment $\mathcal{D}_1$ . . . S15
S10 Posterior distribution for recoil spectroscopy experiment $\mathcal{D}_2$ . . . S16
S11 Posterior distribution for recoil spectroscopy experiment $\mathcal{D}_3$ . . . S17
S12 Posterior distribution for TOF spectroscopy experiment $\mathcal{D}_1$ . . . S18
S13 Posterior distribution for TOF spectroscopy experiment $\mathcal{D}_2$ . . . S19
S14 Posterior distribution for TOF spectroscopy experiment $\mathcal{D}_3$ . . . S20
S15 Bayesian evidence results using recoil spectroscopy ($N_{\text{event}} = 10^1$) . . . S23
S16 Bayesian evidence results using recoil spectroscopy ($N_{\text{event}} = 10^2$) . . . S24
S17 Bayesian evidence results using recoil spectroscopy ($N_{\text{event}} = 10^3$) . . . S25
S18 Bayesian evidence results using recoil spectroscopy ($N_{\text{event}} = 5 \times 10^3$) . . . S26
S19 Bayesian evidence results using TOF spectroscopy ($N_{\text{event}} = 10^1$) . . . S27
S20 Bayesian evidence results using TOF spectroscopy ($N_{\text{event}} = 10^2$) . . . S28
S21 Bayesian evidence results using TOF spectroscopy ($N_{\text{event}} = 10^3$) . . . S29
S22 Bayesian evidence results using TOF spectroscopy ($N_{\text{event}} = 5 \times 10^3$) . . . S30

# List of Supplementary Tables

S1 Performed neutron spectroscopy experiments . . . . . . . . . . . . . . . . . . . . . . . . . . . . . . . S1

# S1 Supplementary Methods

## S1.1 Neutron Spectroscopy Experiments

This supplementary section describes the experimental setup, neutron spectrometer, data reduction pipeline, and neutron background evaluation for the spectroscopy experiments reported in the main study.

### S1.1.1 Experimental Setup

Neutron spectroscopy experiments were performed using an organic glass scintillator (OGS) based spectrometer operating simultaneously in recoil and time-of-flight (TOF) modes. Three independent experiments covered the complete power set of a ${}^{252}_{98}\mathrm{Cf}$ and a ${}^{239}_{94}\mathrm{Pu}$-Be source, hereafter referred to as Cf-252 and PuBe with respective neutron emission rates of $1.74(9) \times 10^6\,\mathrm{s}^{-1}$ and $1.70(4) \times 10^6\,\mathrm{s}^{-1}$. Two additional single-source experiments were performed to generate the spectral templates $\boldsymbol{\psi}$ used in the spectral inversion pipeline (see Sec. S1.2). A summary of all source–detector configurations and live times is provided in Table S1. Experiments were conducted under controlled laboratory conditions at the Detection for Nuclear Nonproliferation Group (DNNG) Lab at the University of Michigan. Reproducible placement of sources and the spectrometer was ensured using an optical breadboard and a custom source holder arc (see Fig. S1). The sources were fixed at a distance of 58.4 cm from the center of the spectrometer's active volume, centered on its horizontal mid-plane, with the azimuthal angle $\varphi$ and an additional 6.8 mm lead sleeve deliberately varied between experiments to test the robustness and generalization capability of the derived template bank (see Sec. S1.2).

**Table S1 Performed neutron spectroscopy experiments.** In this table, we summarize key parameters of the performed neutron spectroscopy experiments.

| Identifier | Source⋆ | $\xi$• $[\mathrm{s}^{-1}]$ | $\varphi$∘ [°] | $t_{\mathrm{live}}$† [s] | Casing‡ |
|---|---|---|---|---|---|
| $\mathcal{D}_1$ | Cf-252 | $1.74(9) \times 10^6$ | +35 | $5.6264 \times 10^4$ | ✗ |
| $\mathcal{D}_2$ | PuBe | $1.70(4) \times 10^6$ | −35 | $1.8000 \times 10^4$ | ✗ |
| $\mathcal{D}_3$ | Cf-252 | $1.74(9) \times 10^6$ | +35 | $2.0293 \times 10^4$ | ✗ |
| | PuBe | $1.70(4) \times 10^6$ | −35 | | ✗ |
| $\mathcal{D}_4$ | Cf-252 | $1.74(9) \times 10^6$ | 0 | $5.5619 \times 10^4$ | ✓ |
| $\mathcal{D}_5$ | PuBe | $1.70(4) \times 10^6$ | 0 | $1.8000 \times 10^4$ | ✓ |
| $\mathcal{D}_\mathrm{b}$ | *background* | | | $5.3159 \times 10^4$ | |

⋆ Deployed neutron source(s), i.e., a sealed Cf-252 spontaneous fission radionuclide source and a sealed PuBe alpha-beryllium source (Pu-239-beryllium oxide with Pu/Be ∼ 0.88 mass ratio).
• Neutron source emission rate.
∘ Azimuth source position with respect to the spectrometer (see Fig. S1).
† Measurement live time (rounded to seconds).
‡ Flag indicating use of a lead sleeve (6.8 mm thickness) around the deployed neutron source(s) (see Fig. S1).

### S1.1.2 Neutron Spectrometer

The neutron spectrometer employed in this work is an organic glass scintillator (OGS) based system that has been characterized extensively in prior studies [1–3]. OGS material offers a com-

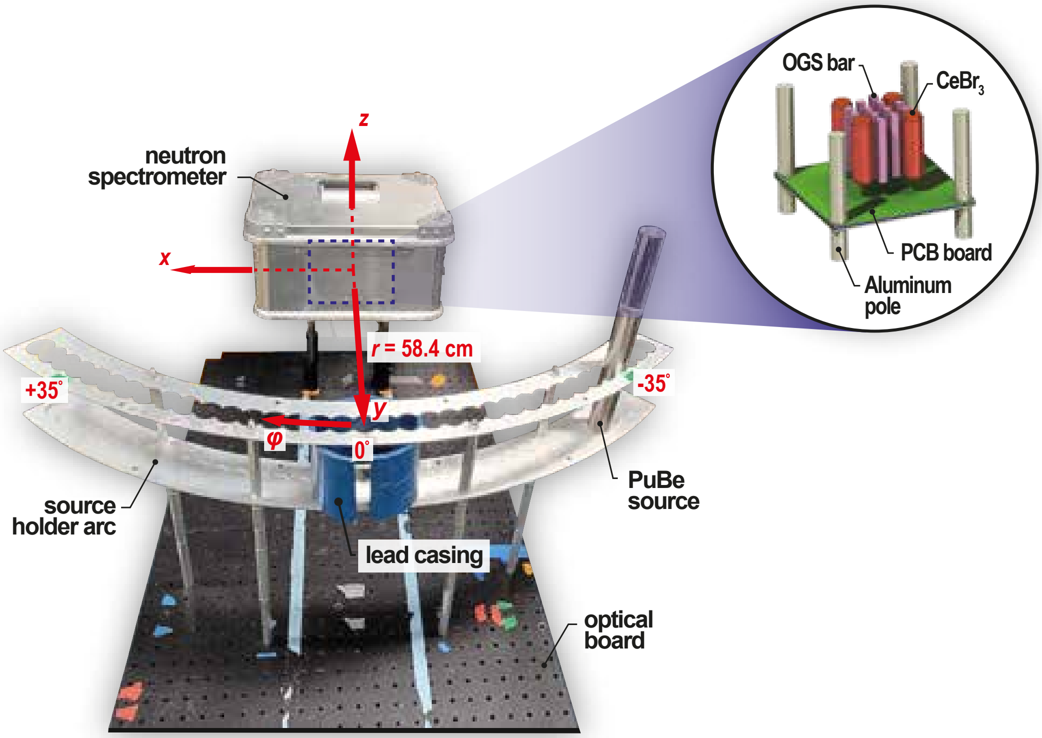


**Figure S1 Experimental setup for neutron spectroscopy.** As an example, we show here the setup for experiment $\mathcal{D}_2$ (single PuBe source at azimuth $\varphi = -35°$ relative to the spectrometer, see Table S1).

bination of high light output, fast scintillation response, and excellent pulse shape discrimination (PSD), making it particularly well suited for neutron spectroscopy across both recoil and TOF modalities [4–6]. The OGS composition used in this work consists of a 90:10 molecular blend of bis(9,9-dimethyl-9H-fluoren-2-yl)diphenylsilane, $C_{42}H_{36}Si$, and phenyltris(9,9-dimethyl-9H-fluorene-2-yl)silane, $C_{51}H_{44}Si$, combined with a 0.2 wt% 1,4-bis(2-methylstyryl)benzene, $C_{24}H_{22}$, wavelength shifter (bis-MSB). Detailed information about the chemistry and synthesis of these compounds can be found in prior work [7].

The spectrometer consists of twelve OGS bars, each with dimensions of $6\times6\times50\,\text{mm}^3$. All bars are wrapped in polytetrafluoroethylene (Teflon) tape to enhance diffuse optical reflection and improve light-collection uniformity. The OGS bars are coupled between two 64-pixel ArrayJ-60035-64P-PCB Onsemi silicon photomultiplier (SiPM) boards operated at 29.6 V. This dual-ended readout configuration allows for event reconstruction on the vertical axis of the OGS bars [1, 8]. Prior work has demonstrated a time resolution of 270 ps at 200–341 keVee between two OGS bars [9]. The spectrometer also features eight encapsulated cylindrical $CeBr_3$ crystals (6 mm diameter and height) for gamma-ray spectroscopy and imaging, which are not relevant for this work. All scintillator–SiPM interfaces are coupled using 0.5 mm thick silicone rubber EJ-560 pads to ensure stable optical transmission. The system uses custom-made printed circuit boards (PCBs) to apply the voltage bias and readout the signals from the SiPM arrays [10]. The signals from all channels are digitized using synchronized CAEN v1730 waveform digitizers (14-bit resolution, 500 MHz sampling rate , 2 V dynamic range). The CAEN v1730 modules were synchronized using a shared

reference clock to maintain consistent timing across boards, enabling accurate reconstruction of inter-bar time differences for TOF analysis. The full detector assembly is enclosed in an aluminum dark box to suppress ambient light. A schematic photograph of the instrument and its mechanical layout is shown in Fig. S1.

### S1.1.3 Data Reduction

In this work, we adopt a benchmarked data reduction pipeline that has already been discussed in detail in our previous work [1, 11]. In this subsection, we limit the discussion to key steps used for recoil and TOF spectroscopy. Further information on waveform processing, filtering, and uncertainty quantification is provided in Refs. [1, 11].

Data are collected in full-waveform acquisition mode with a record length of 800 ns. Energy calibration was performed using $^{137}_{55}Cs$ measurements at the start and end of each experiment, following a calibration protocol described in Ref. [12]. For each detected event, the signals recorded at each end of the organic glass scintillator bar are summed together if triggered within a 20 ns coincidence window. The start time of each detected event is determined by the average of the start times from the paired signals. Neutron and gamma-ray signals were separated using charge-integration pulse shape discrimination (PSD) with an auto-slicing algorithm [13, 14]. This PSD step is applied to all events and is common to both recoil and TOF spectroscopy.

**Recoil Spectroscopy** In recoil spectroscopy mode, we process all PSD-classified neutron events from individual OGS bars. For each event, the scintillation pulse produced by the neutron-induced proton recoil in OGS is integrated to obtain the pulse integral, which quantifies the light output. The calibrated light output is then expressed in electron-equivalent deposited energy to generate the recoil energy spectra.

**TOF Spectroscopy** TOF spectroscopy extends the analysis to multi-bar coincidence events to reconstruct the incident neutron energy. The procedure begins with the same PSD-classified neutron population used for recoil spectroscopy. From this set, candidate TOF events are selected by requiring a two-bar coincidence within a timing window of 0.137–9 ns, motivated by the geometrical constraints of the array and the selected neutron energy band. This filter isolates neutrons that undergo sequential inelastic scattering in two different bars while suppressing accidental coincidences. For each accepted coincidence event, the incident neutron energy $E_0$ is then reconstructed as

$$E_0 = E_{\mathrm{dep},1} + E_{\mathrm{TOF}} \tag{S1}$$

where $E_{\mathrm{dep},1}$ denotes the energy deposited in the first scatter. This quantity is derived from the pulse integral light output and corrected for the non-proportional scintillation response of OGS using the Birks model [3, 15]. The second term, $E_{\mathrm{TOF}}$, represents the neutron energy inferred from the measured inter-bar flight time and the reconstructed interaction positions along each bar [1, 11]. To mitigate systematic biases from gamma-ray leakage, pileup, and geometrically inconsistent scatter sequences, we impose an additional kinematic constraint

$$E_{\mathrm{dep},2} \leq E_{\mathrm{TOF}} \tag{S2}$$

where $E_{\mathrm{dep},2}$ is the energy deposited in the second scatter. This requirement enforces that the second interaction cannot deposit more energy than is kinematically available from the neutron

after the first interaction. Finally, we exclude events for which the relative uncertainty in the reconstructed neutron energy exceeds 50 %, ensuring a high-quality dataset dominated by well-reconstructed trajectories. The reconstructed set of incident neutron energies $\{E_0\}$ is then used to generate the TOF neutron spectra discussed in the main study.

#### S1.1.4 Background Evaluation

A dedicated background run ($\mathcal{D}_b$, see Table S1) without any neutron sources in place was performed to quantify the intrinsic neutron background in both recoil and TOF spectroscopy modes. The measurement configuration, electronics, and acquisition settings were kept identical to the source runs to ensure direct comparability. For each spectroscopy mode, we evaluated the registered background event rates relative to the corresponding gross event rate from all active-source experiments using the data reduction pipeline discussed in Sec. S1.1.3.

Across all measurements, the neutron background was found to be insignificant (see Fig. S2). In recoil mode, the signal-to-background ratio consistently exceeded $10^4$. In TOF mode, where coincidence requirements inherently reduce the gross event rate, the signal-to-background ratio still exceeded $10^3$. No statistically significant structure attributable to background was observed in either the recoil or TOF spectra. Consequently, we conclude that background subtraction is not required for any experiment and the background contribution is negligible for both the spectral template construction and the source-identification analyses.

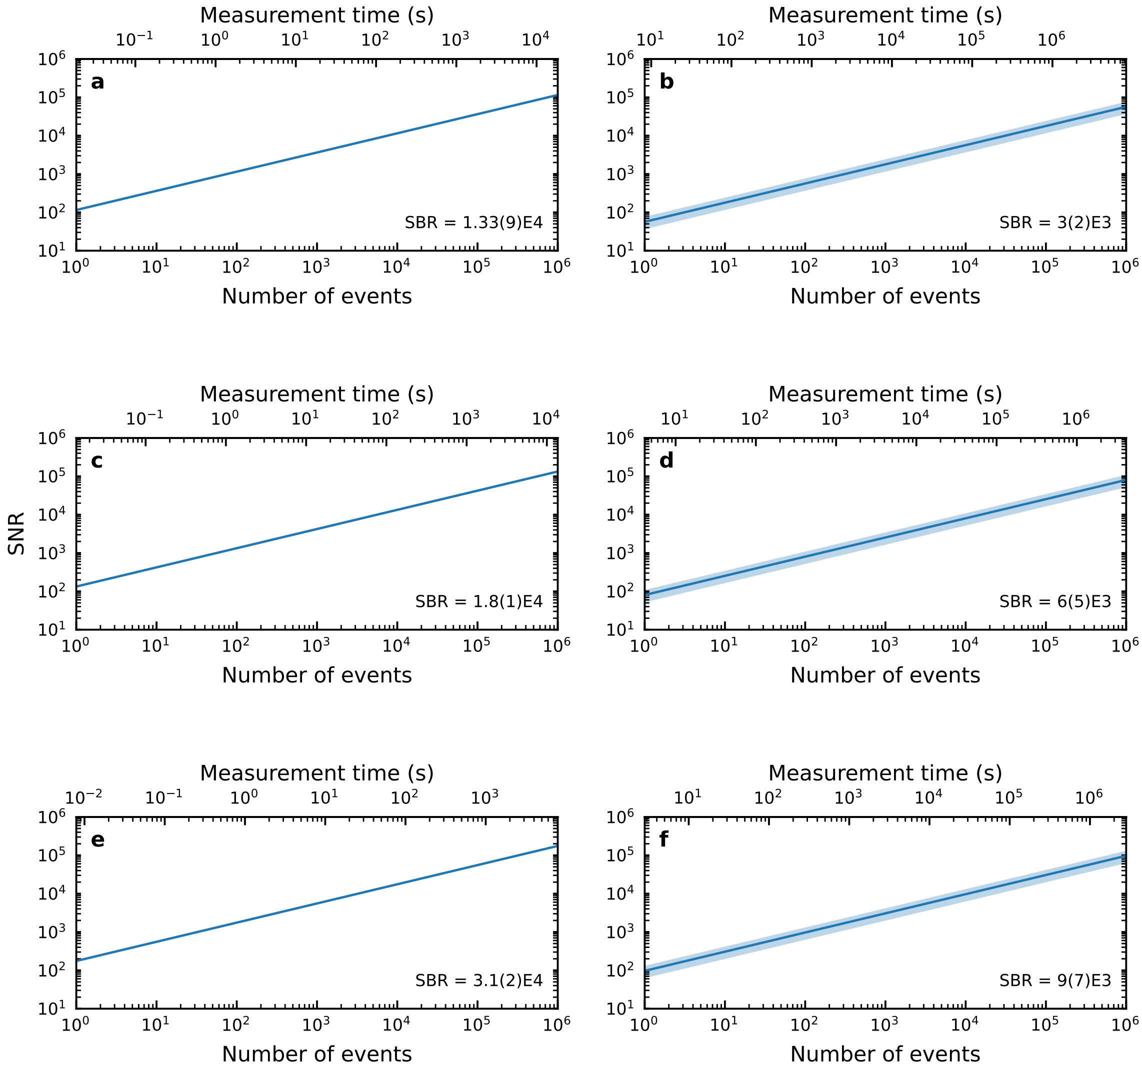


**Figure S2 Background quantification.** Neutron background evaluation quantified by the signal-to-noise ratio (SNR) and signal-to-background ratio (SBR) for recoil spectroscopy (**a**,**c**,**e**) and TOF spectroscopy (**b**,**d**,**f**) as a function of total number of detected events. **a–b** Single-source Cf-252 experiment ($\mathcal{D}_1$). **c–d** Single-source PuBe experiment ($\mathcal{D}_2$). **e–f** Two-source Cf-252 & PuBe experiment ($\mathcal{D}_3$). In addition to the number of detected events, the corresponding measurement times for each experiment are indicated. SNR uncertainties are shown as shaded prediction intervals (coverage factor $k = 1$), while SBR uncertainties are reported in least-significant-figure notation (coverage factor $k = 1$).

## S1.2 Template Bank Generation

In this supplementary method section, we describe the generation of the template bank using generalized additive machine learning models as well as a supplementary assessment of the resulting template bias across different experiments.

### S1.2.1 Generalized Additive Machine Learning Model

As discussed in the main study, we define the source model $\mathcal{M}$ in this work as the discrete ensemble of $S \in \mathbb{N}$ candidate neutron sources together with their associated template set $\mathcal{T} = \{\psi_s\}_{s=1}^{S}$. Each template $\psi_s \in \mathbb{R}_+^N$ represents the normalized full-spectrum response of the spectrometric system with $N \in \mathbb{N}$ channels to the $s$-th neutron source. Following a full-spectrum template matching approach, we then parameterize the forward mapping from any admissible parameter vector $\theta \in \mathbb{R}^M$ to the expected spectral response of a given spectrometric system $\mathcal{M}(\theta) : \Theta \subseteq \mathbb{R}^M \mapsto \mathbb{N}^N$ as the linear superposition of $S \in \mathbb{N}$ spectral templates $\mathcal{M}(\xi) = \sum_{s=1}^{S} \xi_s \, \psi_s$, where $\xi_s \in \mathbb{R}_+$ denotes the corresponding neutron emission rate.

To generate the template bank required to evaluate the full power set of a Cf-252 and PuBe source considered in the main study, we performed two additional single-source Cf-252 ($\mathcal{D}_4$) and PuBe ($\mathcal{D}_5$) calibration experiments, as discussed in Sec. S1.1 (see also Table S1). Adopting a data-driven strategy to minimize model bias, we generated the templates using a generalized additive model (GAM) implemented via the `pyGAM` package [16]. For each source, we inferred a semi-parametric GAM from the calibration data using penalized iteratively reweighted least squares ($10^{-5}$ tolerance). We employed a variable number of $M$ penalized B-spline basis functions ($M \in [30, 70]$ for recoil and $M \in [2, 12]$ for TOF spectroscopy), a Poisson log-link, and a regularization strength $\lambda \in [10^{-1}, 10^3]$. Both the number of basis functions $M$ and the regularization parameter $\lambda$ were selected through hyperparameter tuning. The learned spectral templates, together with the underlying calibration data, are shown in Fig. S3 for recoil and TOF spectroscopy.

### S1.2.2 Template Bias Assessment

To assess the robustness and generalization capability of the spectral template bank, we quantified the spectral bias resulting from controlled variations in source casing and azimuthal orientation between template-generation and identification experiments. Fig. S4 compares the recoil and TOF spectra from repeated single-source measurements of Cf-252 ($\mathcal{D}_1$ vs. $\mathcal{D}_4$) and PuBe ($\mathcal{D}_2$ vs. $\mathcal{D}_5$) (see also Table S1).

For recoil spectroscopy, spectral differences remain small across most of the energy range. A measurable deviation appears only at low deposited energies below 100 keVee, where recoil detection efficiency is most sensitive to geometric and casing-dependent scattering. Above this threshold, recoil spectra exhibit strong reproducibility across all configurations. In contrast, TOF spectroscopy exhibits more pronounced bias at low reconstructed neutron energies. Substantial deviations are observed below 2 MeV, particularly for the Cf-252 experiments, reflecting the increased sensitivity of TOF reconstruction to changes in source–detector geometry and source encapsulation. At higher neutron energies, TOF spectra remain consistent across experiments, indicating stable kinematic reconstruction performance.

Based on this bias assessment, we restricted the energy ranges used for source identification in the main study to 0.1–3.5 MeVee for recoil spectroscopy and 2–10 MeV for TOF spectroscopy. To assess the robustness of this choice, we carried out a supplementary sensitivity analysis in which the lower and upper bounds of each spectral band were varied by ±10 keV. For each modified

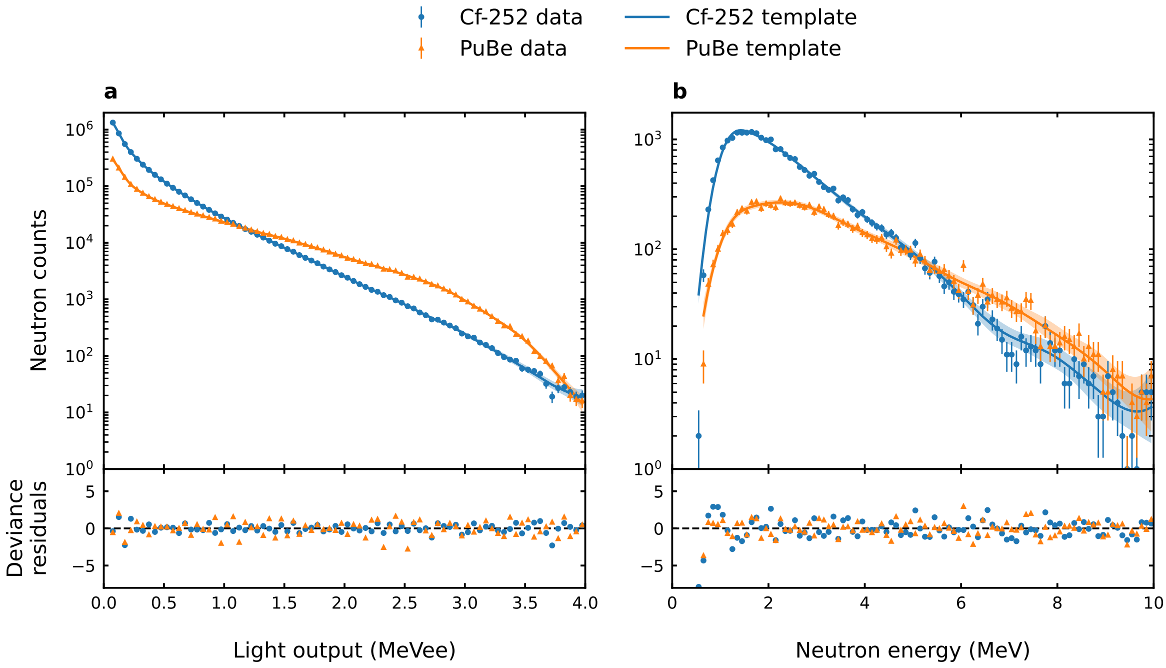


**Figure S3 Generalized additive model (GAM) templates.** Shown are the Cf-252 and PuBe spectral templates together with the corresponding calibration data ($\mathcal{D}_4$ & $\mathcal{D}_5$, see Table S1) for two spectroscopy modalities: **a** Recoil spectroscopy. **b** TOF spectroscopy. Measurement uncertainties are indicated using a coverage factor $k = 1$, while template uncertainties are shown as 99 % prediction intervals. For better interpretability, the spectral templates have been scaled by the neutron emission rate of the respective source to represent absolute neutron counts.

band, we repeated the full Bayesian identification procedure across all measurements and both spectroscopy modalities. The results, shown in Figs. S5–S8, demonstrate that the identification outcomes reported in the main study are stable with respect to mild variations in the selected spectral windows.

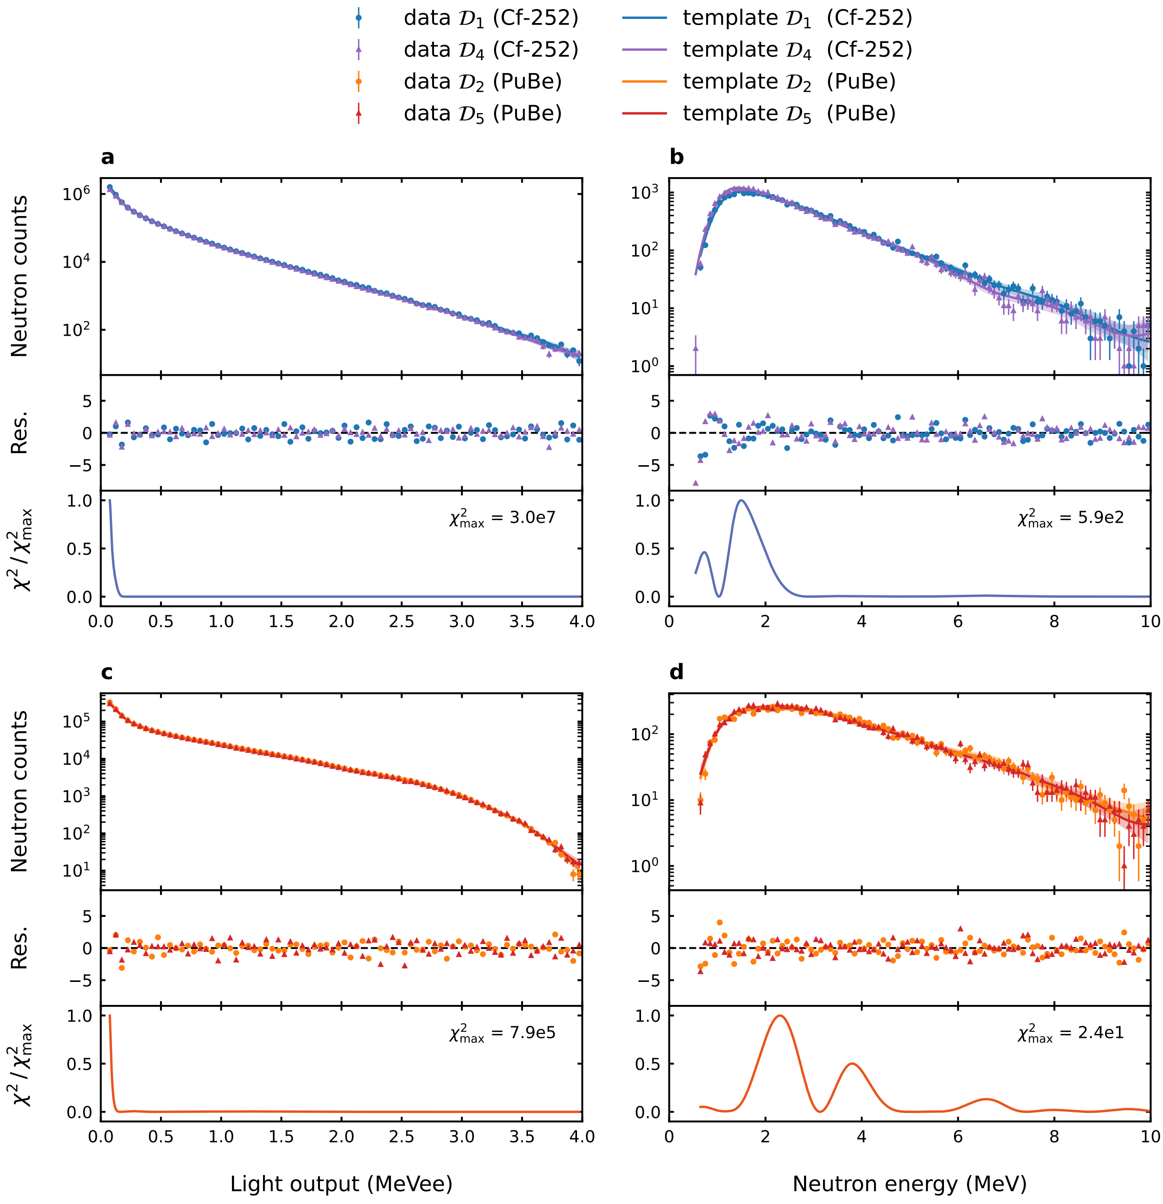


**Figure S4 Template bias quantification.** Results of the spectral template assessment are shown for recoil spectroscopy (**a**,**c**) and TOF spectroscopy (**b**,**d**), evaluated for Cf-252 (**a**,**b**) and PuBe (**c**,**d**) sources. Model bias is quantified using the $\chi^2$ metric, normalized by its maximum value $\chi^2_{\max} := \max \chi^2$ over the evaluated energy range. Measurement uncertainties correspond to a coverage factor $k = 1$, and template uncertainties are shown as 99 % prediction intervals. For better interpretability, the spectral templates have been scaled by the neutron emission rate of the respective source to represent absolute neutron counts.

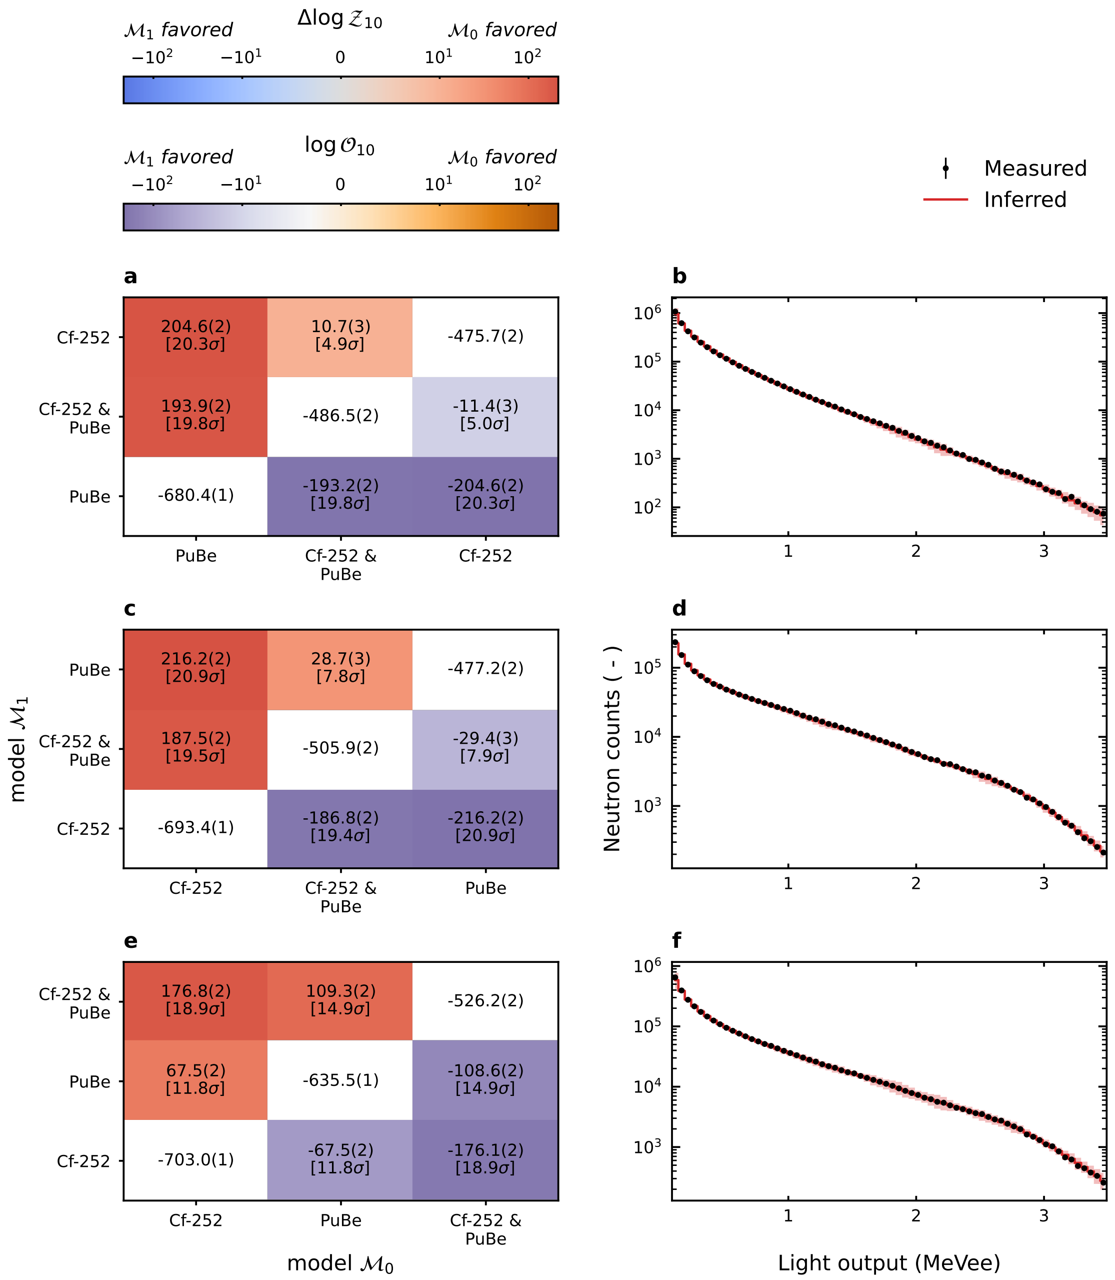


**Figure S5 Bayesian evidence results for three experiments using recoil spectroscopy with 10 keV reduced spectral band (0.09–3.49 MeVee).** (a–b) Single-source Cf-252 experiment ($\mathcal{D}_1$). (c–d) Single-source PuBe experiment ($\mathcal{D}_2$). (e–f) Double-source Cf-252 & PuBe experiment ($\mathcal{D}_3$). Panels (a,c,e) show log evidences $\log\mathcal{Z}_i$ for each model $\mathcal{M}_i$ (diagonal), log Bayes factors $\Delta\log\mathcal{Z}_{10} = \log\mathcal{Z}_1 - \log\mathcal{Z}_0$ (above-diagonal entries), and log posterior odds ratios $\log\mathcal{O}_{10} = \Delta\log\mathcal{Z}_{10} + \log p(\mathcal{M}_1) - \log p(\mathcal{M}_0)$ (below-diagonal entries) with $p(\mathcal{M}) \propto 4^{-\dim(\mathcal{M})}$. Uncertainties are indicated using least-significant-figure notation, with lower statistical-significance bounds in square brackets [17]. Panels (b,d,f) show the measured energy spectra (coverage factor $k = 1$) alongside maximum-a-posteriori predictions and 95 % central posterior predictive intervals (shaded area) for the retrieved (true) source set.

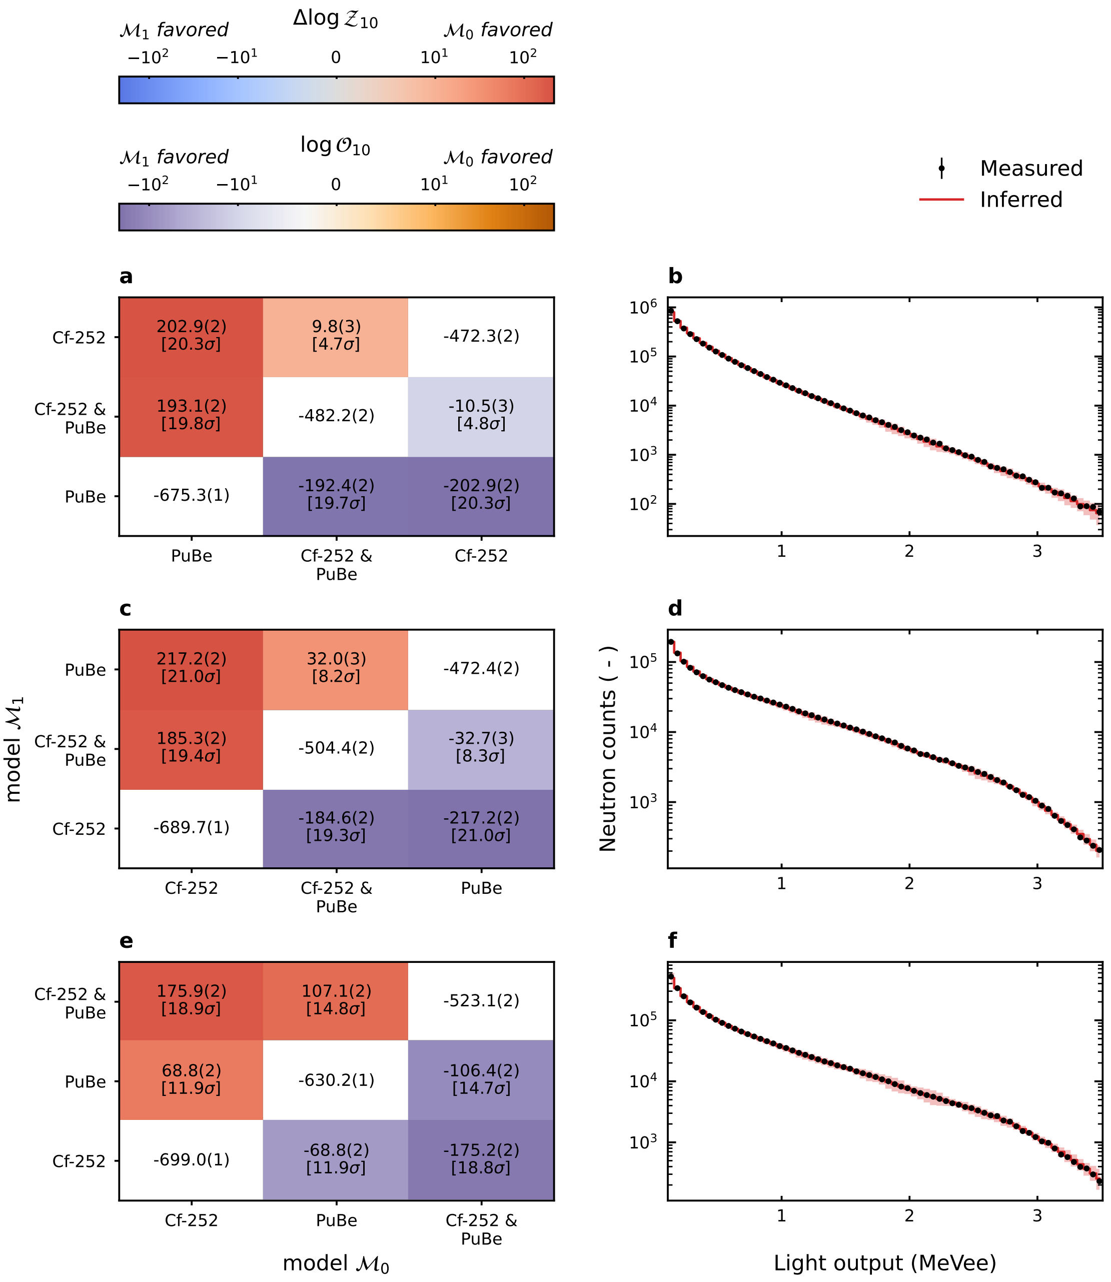


**Figure S6 Bayesian evidence results for three experiments using recoil spectroscopy (10 keV increased spectral band).** Same as Fig. S5 but with 10 keV increased spectral band (0.11–3.51 MeVee).

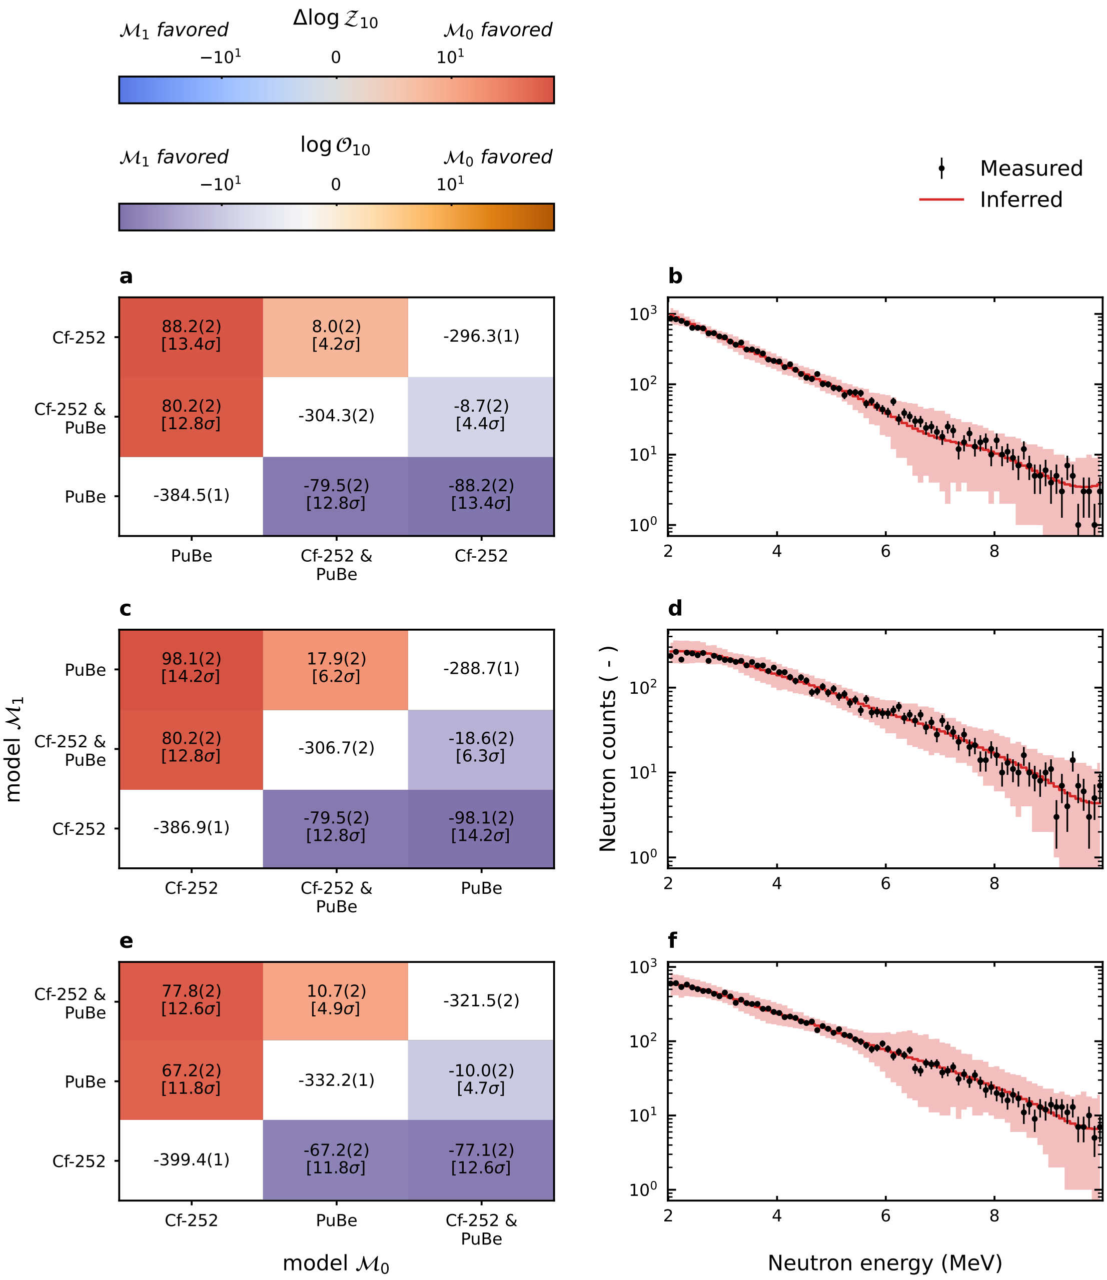


**Figure S7 Bayesian evidence results for three experiments using TOF spectroscopy with 10 keV reduced spectral band.** Same as Fig. S5 but using TOF instead of recoil spectroscopy with 10 keV reduced spectral band (1.99–9.99 MeV).

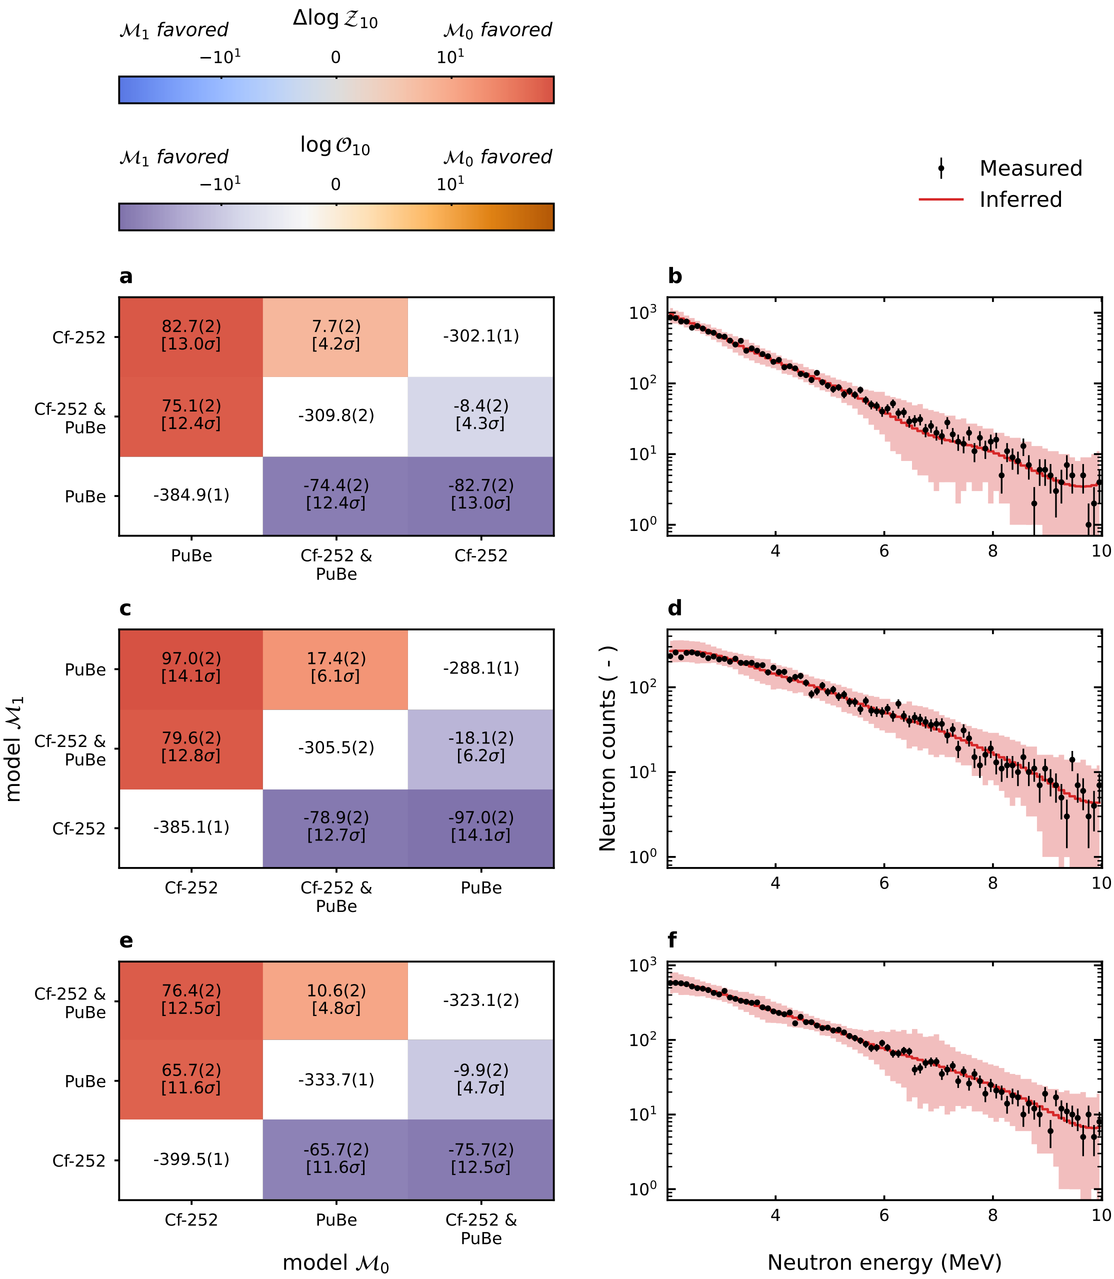


**Figure S8 Bayesian evidence results for three experiments using TOF spectroscopy (10 keV increased spectral band).** Same as Fig. S5 but using TOF instead of recoil spectroscopy with 10 keV increased spectral band (2.01–10.01 MeV).

## S1.3 Bayesian Computations

As discussed in the main study, we establish in this work a Bayesian framework to test a predefined set of competing source models $\{\mathcal{M}_k\}_{k=1}^{K}$ on neutron spectroscopy data $\mathcal{D}$. In this supplementary section, we describe the full Bayesian inference pipeline (including the likelihood and prior specifications) and provide details on the additional Bayesian computations carried out for the event-scale analysis reported in the main study.

### S1.3.1 Bayesian Inference Pipeline

We start our discussion by defining the likelihood function adopted in our Bayesian inference pipeline. As discussed in the main study, we adopted a negative binomial forward model $\boldsymbol{Y} \mid \boldsymbol{\theta} \sim \mathcal{NB}(\mathbf{y} \mid \boldsymbol{\theta})$ to describe the probabilistic mapping from any admissible parameter vector $\boldsymbol{\theta} \in \mathbb{R}^M$ to the spectral response of a given spectrometric system $\mathcal{M}(\boldsymbol{\theta}) : \Theta \subseteq \mathbb{R}^M \mapsto \mathbb{N}^N$, accounting for both measurement uncertainty and overdispersion arising from the experimental process [18–23]. The associated likelihood was formulated using a parameterization established in prior studies [24–26] for a given set of recorded pulse-height spectra $\mathcal{D} = \{\mathbf{y}_i \in \mathbb{N}^N\}_{i=1}^{N_{\mathcal{D}}}$ with $N \in \mathbb{N}$ channels and $N_{\mathcal{D}} \in \mathbb{N}$ realizations as

$$\mathcal{L}(\boldsymbol{\theta}; \mathcal{D}, \mathcal{M}) = \prod_{k=1}^{N_{\mathcal{D}}} \prod_{j=1}^{N} \frac{\Gamma\left(y_{k,j} + \frac{1}{\alpha}\right)}{\Gamma\left(\frac{1}{\alpha}\right)\Gamma\left(y_{k,j}+1\right)} \left(\frac{1}{1+\alpha\mathcal{M}(\boldsymbol{\xi})}\right)^{\frac{1}{\alpha}} \left(\frac{1}{1+[\alpha\mathcal{M}(\boldsymbol{\xi})]^{-1}}\right)^{y_{k,j}} \tag{S3}$$

with $\Gamma(\cdot)$ denoting the gamma function and $\mathcal{M}(\cdot)$ the deterministic forward operator introduced in the main study, mapping neutron emission rates $\boldsymbol{\xi} \in \mathbb{R}_+^S$ for a model containing $S$ sources/templates to expected counts $y_{k,j} \in \mathbb{N}$ (see also Sec. S1.2). The dispersion parameter $\alpha \in \mathbb{R}_+$ in Eq. S3 controls the overdispersion beyond the intrinsic Poisson statistics as $\mathrm{Var}(\boldsymbol{Y}) = \langle \boldsymbol{Y} \rangle + \alpha \langle \boldsymbol{Y} \rangle^2$ with $\alpha \in \mathbb{R}_+$. To prevent biased inference, we incorporated the dispersion parameter $\alpha$ directly into the inference procedure, estimating it concurrently with the source emission rates. As a result, the inverse problem associated with a given model $\mathcal{M}$ became $M = S + 1$ dimensional, with the full parameter vector defined as $\boldsymbol{\theta} := (\boldsymbol{\xi}, \alpha)$.

It is important to note that the gamma function terms in Eq. S3 increase rapidly for moderately large arguments, requiring careful numerical evaluation of the likelihood function. To prevent overflow, we worked with the logarithm of the likelihood function:

$$\begin{aligned}\log \mathcal{L}(\boldsymbol{\theta}; \mathcal{D}, \mathcal{M}) = \sum_{k=1}^{N_{\mathcal{D}}} \sum_{j=1}^{N} \log\Gamma\left(y_{k,j} + \frac{1}{\alpha}\right) - \log\Gamma\left(\frac{1}{\alpha}\right) - \log\Gamma\left(y_{k,j}+1\right) \\ - \frac{1}{\alpha}\log\left(1+\alpha\mathcal{M}(\boldsymbol{\xi})\right) - y_{k,j}\log\left(1+\frac{1}{\alpha\mathcal{M}(\boldsymbol{\xi})}\right)\end{aligned} \tag{S4}$$

commonly referred to as the log-likelihood [27]. The log-gamma terms in Eq. S4 were computed using a numerically robust algorithm [28, 29], which maintains stability and precision across the full dynamic range of input arguments.

The likelihood specifications in Eqs. S3 and S4 form the first element of the Bayesian pipeline. Completing the posterior model requires assigning suitable priors to the model parameters $\boldsymbol{\theta}$. To avoid overly restrictive assumptions on these priors, we adopted weakly informative, statistically independent marginal priors $p(\boldsymbol{\theta}) := \prod_{i=1}^{M} p\left(\theta_i\right)$ for all model parameters $\theta$, with the marginal

priors $p(\theta)$ defined based on the principle of maximum entropy [30]. Specifically, we chose a truncated normal distribution for the neutron emission rate $\xi \sim \mathcal{N}(\mu = 10^8, \sigma = 10^8) \in [0, \infty)$, invariant with respect to the source, and an exponential distribution for the dispersion parameter $\alpha \sim \mathcal{E}(\lambda = 1) \in [0, \infty)$. It is worth noting that, in accordance with the Bayesian framework, prior knowledge of the spectral template bias was explicitly incorporated by imposing a lower bound on the dispersion parameter as $\alpha + \Delta\mathbf{y}^2/\mathbf{y}^2$, where $\Delta\mathbf{y}$ was informed by the template bias quantification presented in Sec. S1.2.

Using the specified joint prior distribution and likelihood function, we evaluated the marginal likelihood $\mathcal{Z} := p(\mathcal{D} \mid \mathcal{M})$ while simultaneously sampling the posterior distribution $p(\theta \mid \mathcal{D}, \mathcal{M})$ using the nested sampling implementation `dynesty` (version `3.0.0`) [31]. This Bayesian inference procedure was carried out independently for each candidate source model $\{\mathcal{M}_k\}_{k=1}^{K}$, yielding a corresponding set of Bayesian evidence values $\{\mathcal{Z}_k\}_{k=1}^{K}$ from which Bayes factors and posterior odds ratios are computed (see main study). For each nested-sampling run, we used $2^{10}$ live points and set the evidence tolerance to $\Delta \log \mathcal{Z} = 0.1$. The bounding strategy `single` was adopted, and new samples were drawn using the default uniform-sampling method. All other sampler settings were kept at their default values. Convergence and numerical precision were evaluated using established nested-sampling diagnostics [31–33]. Across all runs, we obtained an effective sample size ESS $> 4 \times 10^3$ and a sampling efficiency exceeding 25 %. Following the uncertainty quantification framework introduced in Refs. [32, 34, 35], the statistical uncertainties on the computed Bayesian evidence values were estimated directly from the `dynesty` outputs and are reported in the main study.

In addition to the Bayesian evidence values, Bayes factors, and posterior odds ratios reported in the main study, we provide the full posterior results for the nested sampling runs of the true source models in Figs. S9–S11 for recoil spectroscopy and in Figs. S12–S14 for TOF spectroscopy. As expected, the posterior predictions of neutron emission rates exhibit a systematic bias arising from the adopted template bank with varied source positions and casings (see Sec. S1.2). However, this bias remains statistically insignificant at the 99 % credible interval, indicating that the template bank generalizes not only for model selection but also, to a limited extent, for parameter inference under the considered source–detector configurations.

From the full posterior results in Figs. S9–S14, we also identify systematic differences in the dispersion parameter $\alpha$ between recoil and TOF spectroscopy across all experiments. For recoil spectroscopy, the posterior medians and corresponding 95 % central credible intervals are $\alpha = (1.7^{+4.2}_{-1.5} \times 10^{-4}, 1.5^{+2.5}_{-1.2} \times 10^{-4}, 4.4^{+24.5}_{-4.2} \times 10^{-5})$, whereas TOF spectroscopy yields substantially larger values, $\alpha = (1.5^{+3.6}_{-1.5} \times 10^{-3}, 1.3^{+4.5}_{-1.2} \times 10^{-3}, 8.0^{+28.0}_{-5.2} \times 10^{-4})$, for the experiments $(\mathcal{D}_1, \mathcal{D}_2, \mathcal{D}_3)$ (see Table S1). These results demonstrate that TOF spectroscopy exhibits a dispersion parameter whose posterior median exceeds that of recoil spectroscopy by roughly an order of magnitude across all source–detector configurations. This pronounced increase in $\alpha$ implies a significantly larger event-by-event statistical variance relative to the mean, consistent with the behavior expected for neutron-counting processes governed by overdispersion. In turn, the enhanced overdispersion directly reduces the effective information carried by each recorded event. This finding provides a quantitative basis for the reduced information-gain scaling observed for TOF spectroscopy in the main study, thereby reinforcing the interpretation that overdispersion constitutes the dominant statistical limitation in TOF-based inference under the examined experimental conditions.

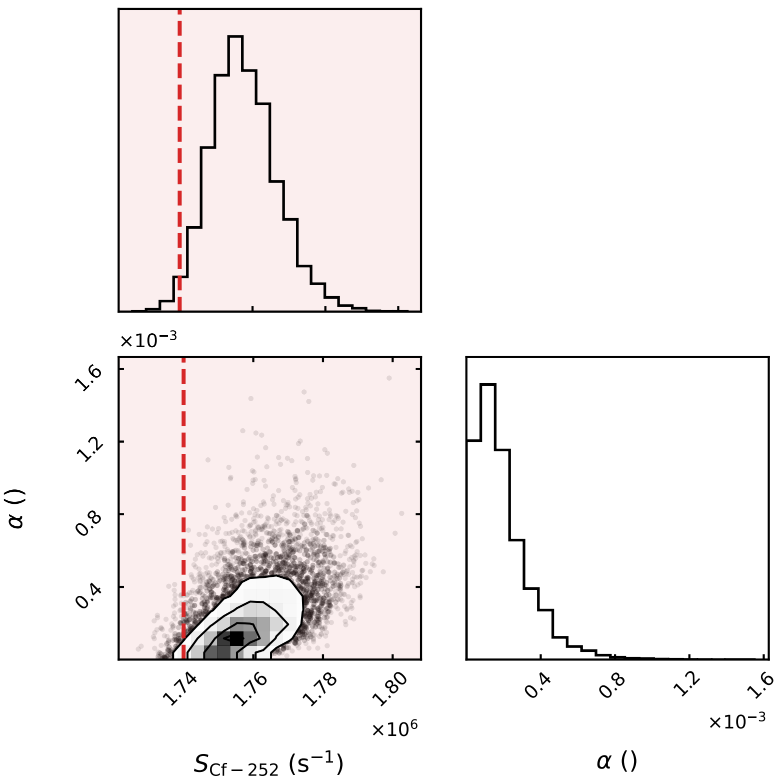


**Figure S9 Posterior distribution for recoil spectroscopy experiment $\mathcal{D}_1$.** Here, we present the posterior distribution of the neutron emission rate ($\xi_{\text{Cf-252}}$) and negative binomial dispersion parameter ($\alpha$) associated with the inferred (true) source set for the recoil spectroscopy experiment $\mathcal{D}_1$ (see Table S1). The true neutron emission rate is indicated by the red dashed line (3-sigma red shaded area bound). For the two-dimensional marginal posteriors, we indicate the (11.8 %, 39.3 %, 67.5 %, 86.4 %) central credible regions by solid black isolines, corresponding to (0.5, 1, 1.5, 2)-sigma credible regions for a two-dimensional Gaussian distribution [36].

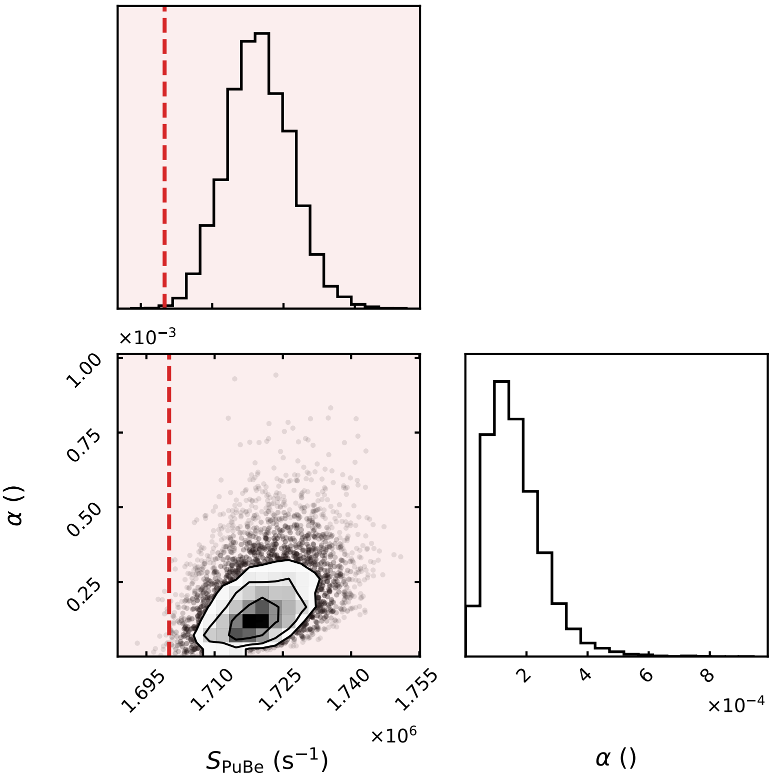


**Figure S10** **Posterior distribution for recoil spectroscopy experiment $\mathcal{D}_2$.** Here, we present the posterior distribution of the neutron emission rate ($\xi_{\mathrm{PuBe}}$) and negative binomial dispersion parameter ($\alpha$) associated with the inferred (true) source set for the recoil spectroscopy experiment $\mathcal{D}_2$ (see Table S1). The true neutron emission rate is indicated by the red dashed line (3-sigma red shaded area bound). For the two-dimensional marginal posteriors, we indicate the (11.8 %, 39.3 %, 67.5 %, 86.4 %) central credible regions by solid black isolines, corresponding to (0.5, 1, 1.5, 2)-sigma credible regions for a two-dimensional Gaussian distribution [36].

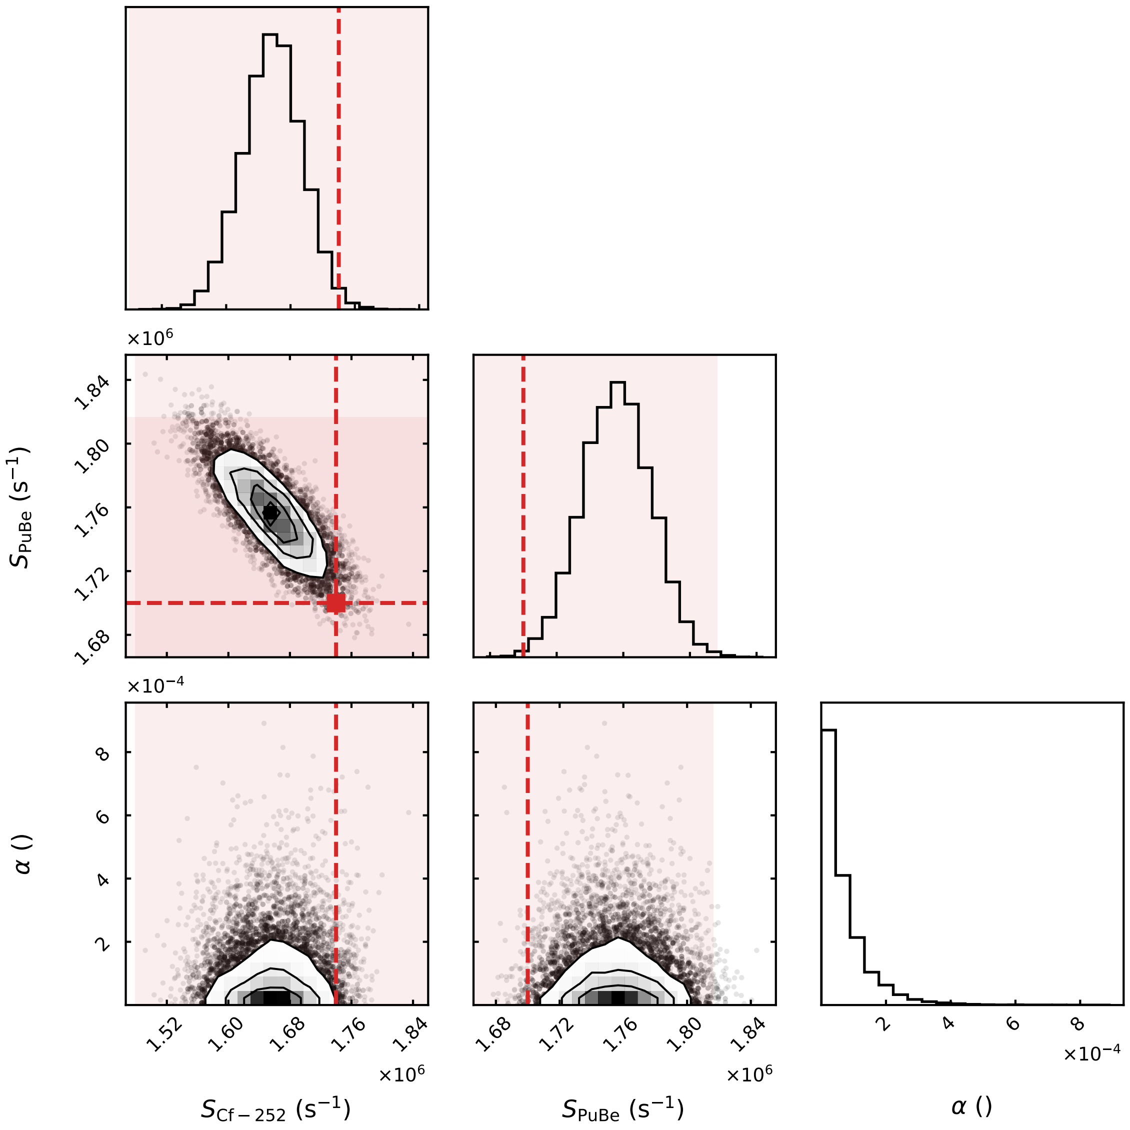


**Figure S11 Posterior distribution for recoil spectroscopy experiment $\mathcal{D}_3$.** Here, we present the posterior distribution of the neutron emission rates ($\xi_{\mathrm{Cf-252}}$ & $\xi_{\mathrm{PuBe}}$) and negative binomial dispersion parameter ($\alpha$) associated with the inferred (true) source set for the recoil spectroscopy experiment $\mathcal{D}_3$ (see Table S1). The true neutron emission rates are indicated by the red dashed line (3-sigma red shaded area bound). For the two-dimensional marginal posteriors, we indicate the (11.8 %, 39.3 %, 67.5 %, 86.4 %) central credible regions by solid black isolines, corresponding to (0.5, 1, 1.5, 2)-sigma credible regions for a two-dimensional Gaussian distribution [36].

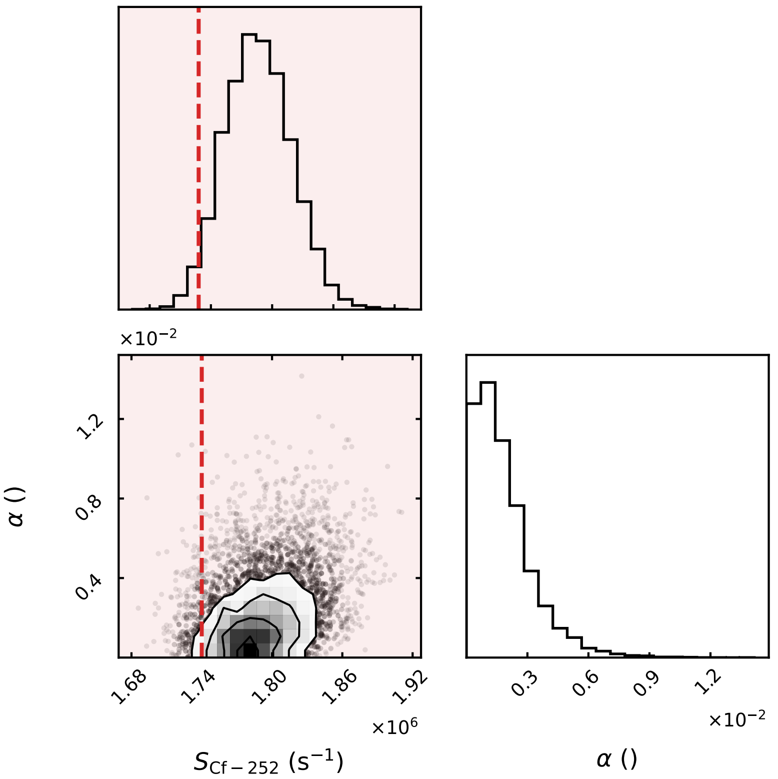


**Figure S12 Posterior distribution for TOF spectroscopy experiment $\mathcal{D}_1$.** Same as Fig. S9, but using TOF spectroscopy instead of recoil spectroscopy.

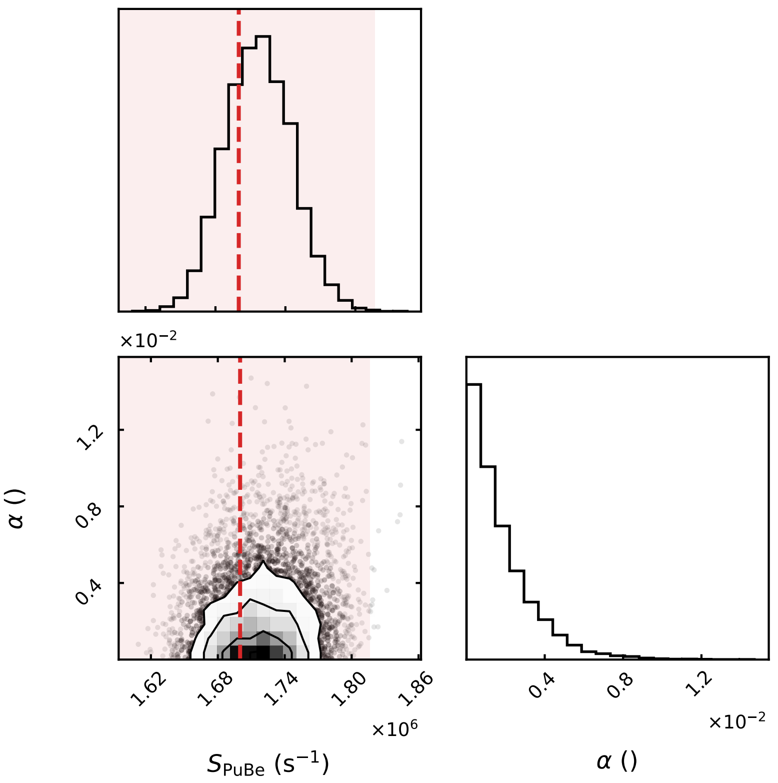


**Figure S13 Posterior distribution for TOF spectroscopy experiment $\mathcal{D}_2$.** Same as Fig. S10, but using TOF spectroscopy instead of recoil spectroscopy.

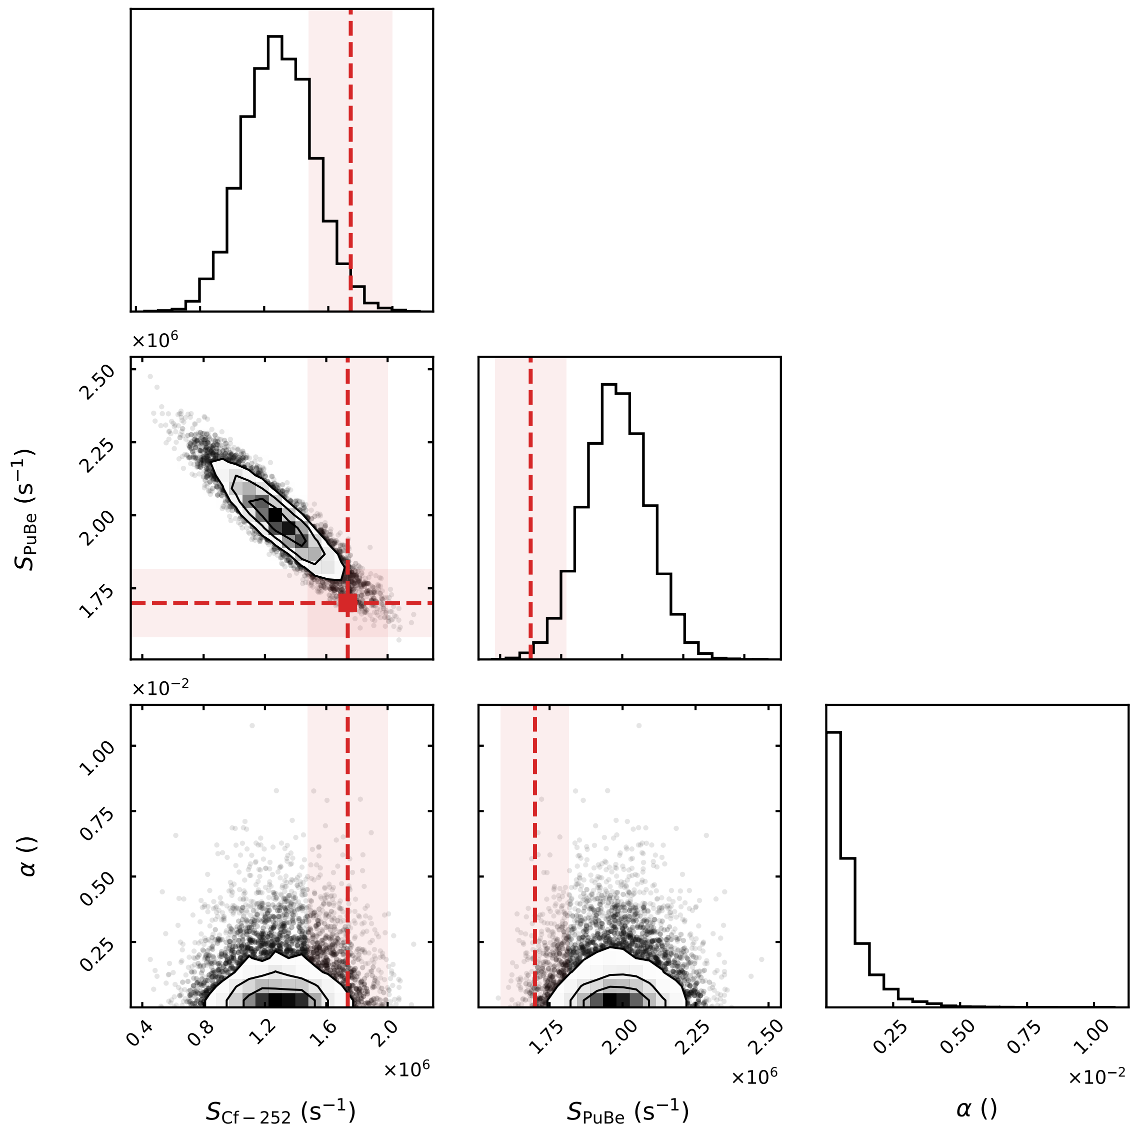


**Figure S14 Posterior distribution for TOF spectroscopy experiment $\mathcal{D}_3$.** Same as Fig. S11, but using TOF spectroscopy instead of recoil spectroscopy.

### S1.3.2 Event Scaling

In the main study, we reported additional Bayesian scaling results, specifically how the posterior model probability $p(\mathcal{M}_{\mathrm{true}} \mid \mathcal{D})$ and the relative entropy $\mathcal{IG}(\mathcal{M}_{\mathrm{true}};\mathcal{D})$, both conditioned on the true source model $\mathcal{M}_{\mathrm{true}}$, scale with the number of detected events for the experiments based on recoil and TOF spectroscopy. In this section, we detail the computational procedure used to obtain these quantities.

We started by generating a collection of resampled pulse-height spectra $\{\mathcal{D}^{(b)}\}_{b=1}^{B}$, where each $\mathcal{D}^{(b)} \in \mathbb{N}^N$ contained exactly $N_{\mathrm{event}}^{(b)}$ total counts drawn from a predefined reference dataset $\mathcal{D} = \{\mathbf{y} \in \mathbb{N}^N\}$ corresponding to one of the datasets discussed in Sec. S1.1. Defining the spectral probabilities $p_i = y_i \big/ \sum_{j=1}^{N} y_j$, each spectrum was generated via multinomial sampling $\mathbf{y}^{(b)} \sim \mathrm{Multinomial}( N_{\mathrm{event}}^{(b)}, \mathbf{p}) \in \mathbb{N}^N$ with probabilities $p_i$ proportional to the reference spectrum $\mathcal{D}$. This procedure yielded independent finite-statistics realizations that preserve the spectral shape of $\mathcal{D}$. For each number of events $N_{\mathrm{event}}^{(b)}$, we generated $N_{\mathrm{rep}} = 10^3$ realizations, with $N_{\mathrm{event}}^{(b)}$ defined on a logarithmically spaced grid with 400 instances between $N_{\mathrm{event}}^{(1)} = 1$ and $N_{\mathrm{event}}^{(B)} = N_{\mathrm{event}}$, with $N_{\mathrm{event}}$ being the number of detected events in $\mathcal{D}$.

We continued by computing the log Bayesian evidence $\log \mathcal{Z}^{(b)}$ for each resampled spectrum $\mathcal{D}^{(b)}$ as

$$
\begin{aligned}
\log \mathcal{Z}^{(b)} &= \log \int_{\Theta} \mathcal{L}\left(\mathcal{D}^{(b)}|\theta,\mathcal{M}\right) p\left(\theta|\mathcal{M}\right) \mathrm{d}\theta && \text{(S5a)}\\
&= \log \int_{\Theta} \mathcal{L}\left(\mathcal{D}^{(b)}|\theta,\mathcal{M}\right) p\left(\theta|\mathcal{M}\right) \underbrace{\frac{\mathcal{L}(\mathcal{D}|\theta,\mathcal{M})\, p\left(\theta|\mathcal{M}\right)}{\mathcal{Z}}}_{p(\theta|\mathcal{D},\mathcal{M})} \frac{\mathcal{Z}}{\mathcal{L}(\mathcal{D}|\theta,\mathcal{M})\, p\left(\theta|\mathcal{M}\right)} \mathrm{d}\theta && \text{(S5b)}\\
&= \log \mathcal{Z} - \log \int_{\Theta} \underbrace{\frac{\mathcal{L}\left(\mathcal{D}^{(b)}|\theta,\mathcal{M}\right)}{\mathcal{L}(\mathcal{D}|\theta,\mathcal{M})}}_{\text{likelihood ratio}} \underbrace{p\left(\theta|\mathcal{D},\mathcal{M}\right)}_{\text{posterior}} \mathrm{d}\theta && \text{(S5c)}\\
&\approx \log \mathcal{Z} - \log N_{\theta} + \log \sum_{i=1}^{N_{\theta}} \exp\left[\log \mathcal{L}\left(\mathcal{D}^{(b)}|\theta_i,\mathcal{M}\right) - \log \mathcal{L}\left(\mathcal{D}|\theta_i,\mathcal{M}\right)\right] && \text{(S5d)}
\end{aligned}
$$

with $\log \mathcal{Z}$ denoting the log Bayesian evidence of the reference dataset $\mathcal{D}$, while $\log \mathcal{L}(\mathcal{D}^{(b)} \mid \theta_i, \mathcal{M})$ and $\log \mathcal{L}(\mathcal{D} \mid \theta_i, \mathcal{M})$ are the log likelihoods evaluated at each posterior sample $\{\theta_i\}_{i=1}^{N_\theta}$ obtained from the `dynesty` runs for a given reference dataset $\mathcal{D}$ and source model $\mathcal{M}$ (see Sec. S1.3.1). The importance sampling procedure in Eq. S5d allowed us to efficiently estimate the log Bayesian evidence for each of the $400 \times 1000$ resampled spectra, from which we then computed the mean and standard error using Monte Carlo error propagation across the $N_{\mathrm{rep}} = 1000$ realizations.

Based on the computed set of log Bayesian evidence values $\log \mathcal{Z}^{(b)}$ for each resampled spectrum $\mathcal{D}^{(b)}$, we computed the posterior model probability, i.e., the posterior probability $p(\mathcal{M}_{\mathrm{true}} \mid \mathcal{D}^{(b)})$ of retrieving the true source model $\mathcal{M}_{\mathrm{true}}$ conditioned on the resampled data $\mathcal{D}^{(b)}$ and a set of competing models $\{\mathcal{M}_k\}_{k=1}^{K}$ with associated model priors $p(\mathcal{M}_k)$:

$$
p\left(\mathcal{M}_{\mathrm{true}}|\mathcal{D}^{(b)}\right) = \frac{p\left(\mathcal{D}^{(b)}|\mathcal{M}_{\mathrm{true}}\right) p\left(\mathcal{M}_{\mathrm{true}}\right)}{\sum_{k=1}^{K} p\left(\mathcal{D}^{(b)}|\mathcal{M}_k\right) p\left(\mathcal{M}_k\right)} \qquad \text{(S6)}
$$

with $p(\mathcal{D}^{(b)} \mid \mathcal{M}_k) = \mathcal{Z}_k^{(b)}$ denoting the Bayesian evidence of the resampled data $\mathcal{D}^{(b)}$ conditioned on the model $\mathcal{M}_k$. For numerical stability, Eq. S6 was evaluated in logarithmic form using the

LogSumExp (LSE) transformation, which allows for robust computation of the logarithm of a sum of exponentials and prevents overflow or underflow:

$$\log p\left(\mathcal{M}_{\text{true}}|\mathcal{D}^{(b)}\right)=\log \mathcal{Z}_{\text{true}}^{(b)}+\log p\left(\mathcal{M}_{\text{true}}\right)-\log\sum_{k=1}^{K}\exp\left[\log \mathcal{Z}_{k}^{(b)}+\log p\left(\mathcal{M}_{k}\right)\right] \tag{S7}$$

where $\mathcal{Z}_{\text{true}}^{(b)} := p(\mathcal{D}^{(b)} \mid \mathcal{M}_{\text{true}})$ denotes the Bayesian evidence of the resampled data $\mathcal{D}^{(b)}$ conditioned on the true model $\mathcal{M}_{\text{true}}$. As with the Bayesian evidence itself, the statistical uncertainty in the posterior model probability $p(\mathcal{M}_{\text{true}} \mid \mathcal{D}^{(b)})$ was quantified via Monte Carlo error propagation over the $N_{\text{rep}} = 10^3$ available realizations.

Using the posterior model probabilities, we quantified the information gain (relative entropy) associated with identifying the true source model $\mathcal{M}_{\text{true}}$. For each resampled spectrum $\mathcal{D}^{(b)}$, the information gain was computed as the Kullback–Leibler divergence between the posterior and prior probabilities for the true model:

$$\mathcal{IG}\left(\mathcal{M}_{\text{true}};\mathcal{D}^{(b)}\right)=p\left(\mathcal{M}_{\text{true}} \mid \mathcal{D}^{(b)}\right)\log_2\frac{p\left(\mathcal{M}_{\text{true}} \mid \mathcal{D}^{(b)}\right)}{p\left(\mathcal{M}_{\text{true}}\right)}, \tag{S8}$$

where $p(\mathcal{M}_{\text{true}} \mid \mathcal{D}^{(b)})$ is the posterior model probability computed in log-space using the LSE transformation (see Eq. S7) to ensure numerical stability. This formulation quantifies the information gained about the true model from the observed data relative to the prior expectation. The statistical uncertainty in $\mathcal{IG}$ was again estimated by propagating the Monte Carlo variability across the $N_{\text{rep}} = 10^3$ realizations of the resampled spectra. Averaging over these realizations yielded the mean information gain and its standard error, providing a robust measure of how strongly each dataset supports the true model under the competing hypothesis set $\{\mathcal{M}_k\}_{k=1}^{K}$.

In addition to the scaling results presented in the main study, we further evaluated Bayes factors, posterior odds ratios, and posterior predictive distributions for a representative subset of resampled spectra, specifically those with $N_{\text{event}}^{(b)} \in \{10^1, 10^2, 10^3, 5\times 10^3\}$ events. These analyses were performed to corroborate the scaling results and provide additional verification of the Bayesian inference pipeline. The corresponding supplementary results are shown in Figs. S15–S22, and they reproduce the expected physical and statistical trends across all experiments and spectroscopy modalities. At low event counts, the data contain insufficient information to discriminate between competing source models. As the number of detected events increases, the spectral data become progressively more informative, and the posterior probability converges toward the true source model, consistent with the trends observed in the main study.

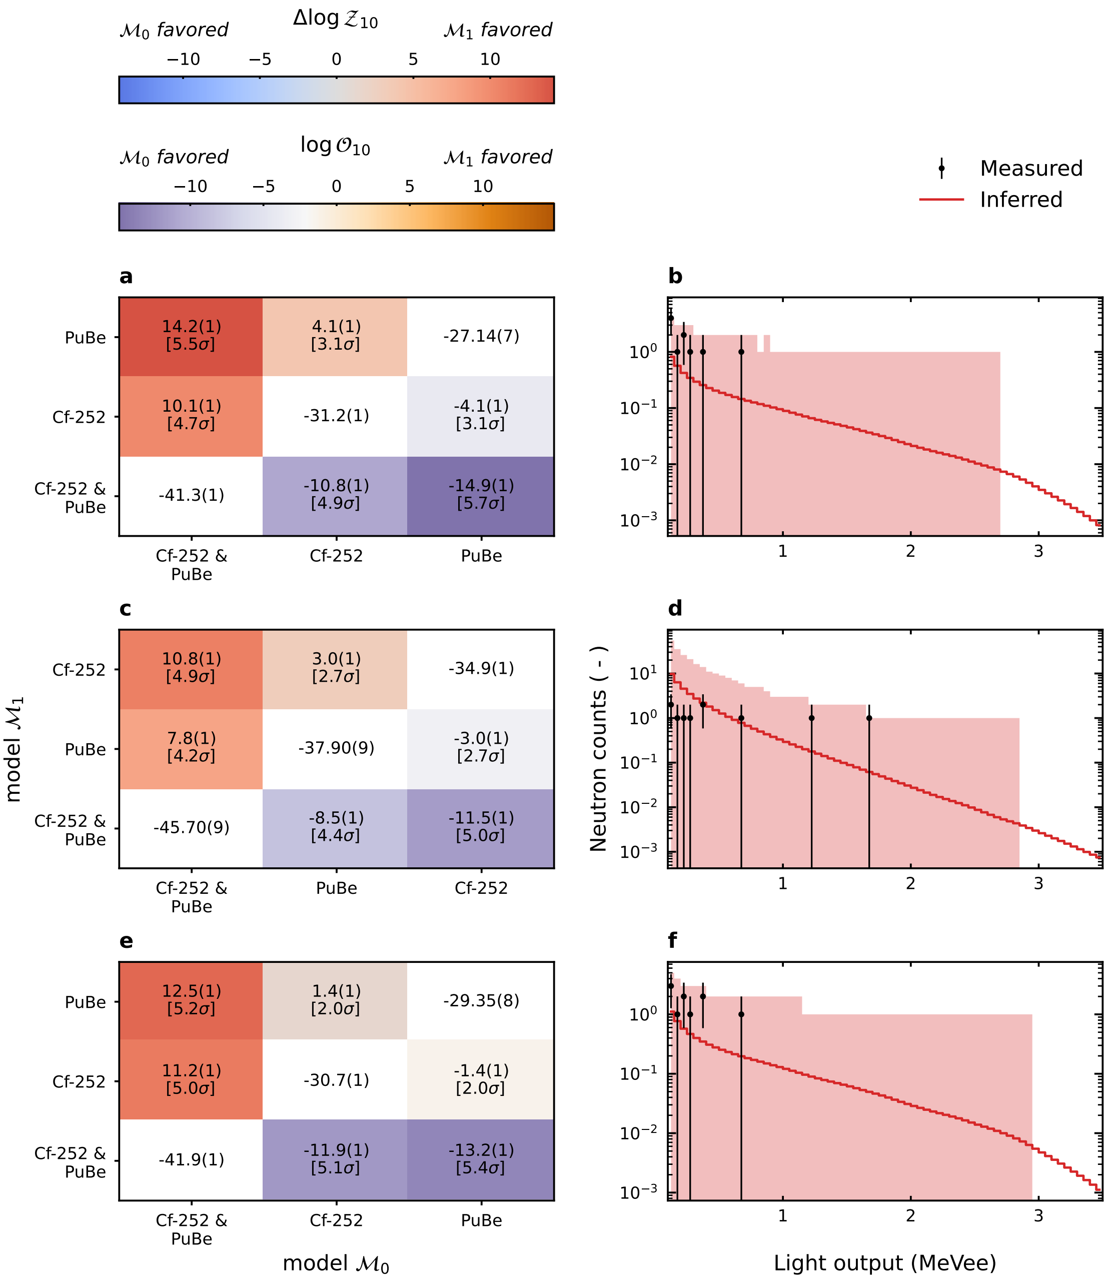


**Figure S15 Bayesian evidence results for three experiments using recoil spectroscopy with $N_{\text{event}} = 10^1$.** (a–b) Single-source Cf-252 experiment ($\mathcal{D}_1$). (c–d) Single-source PuBe experiment. (e–f) Double-source Cf-252 & PuBe experiment. Panels (a,c,e) show log evidence values $\log\mathcal{Z}_i$ for each model $\mathcal{M}_i$ (diagonal), log Bayes factors $\Delta\log\mathcal{Z}_{10} = \log\mathcal{Z}_1 - \log\mathcal{Z}_0$ (above-diagonal entries), and log posterior odds ratios $\log\mathcal{O}_{10} = \Delta\log\mathcal{Z}_{10} + \log p(\mathcal{M}_1) - \log p(\mathcal{M}_0)$ (below-diagonal entries) with $p(\mathcal{M}) \propto 4^{-\dim(\mathcal{M})}$. Uncertainties are indicated using least-significant-figure notation, with lower statistical-significance bounds in square brackets [17]. Panels (b,d,f) show the measured energy spectra (coverage factor $k = 1$) alongside maximum-a-posteriori predictions and 95 % central posterior predictive intervals (shaded area) for the retrieved (true) source set.

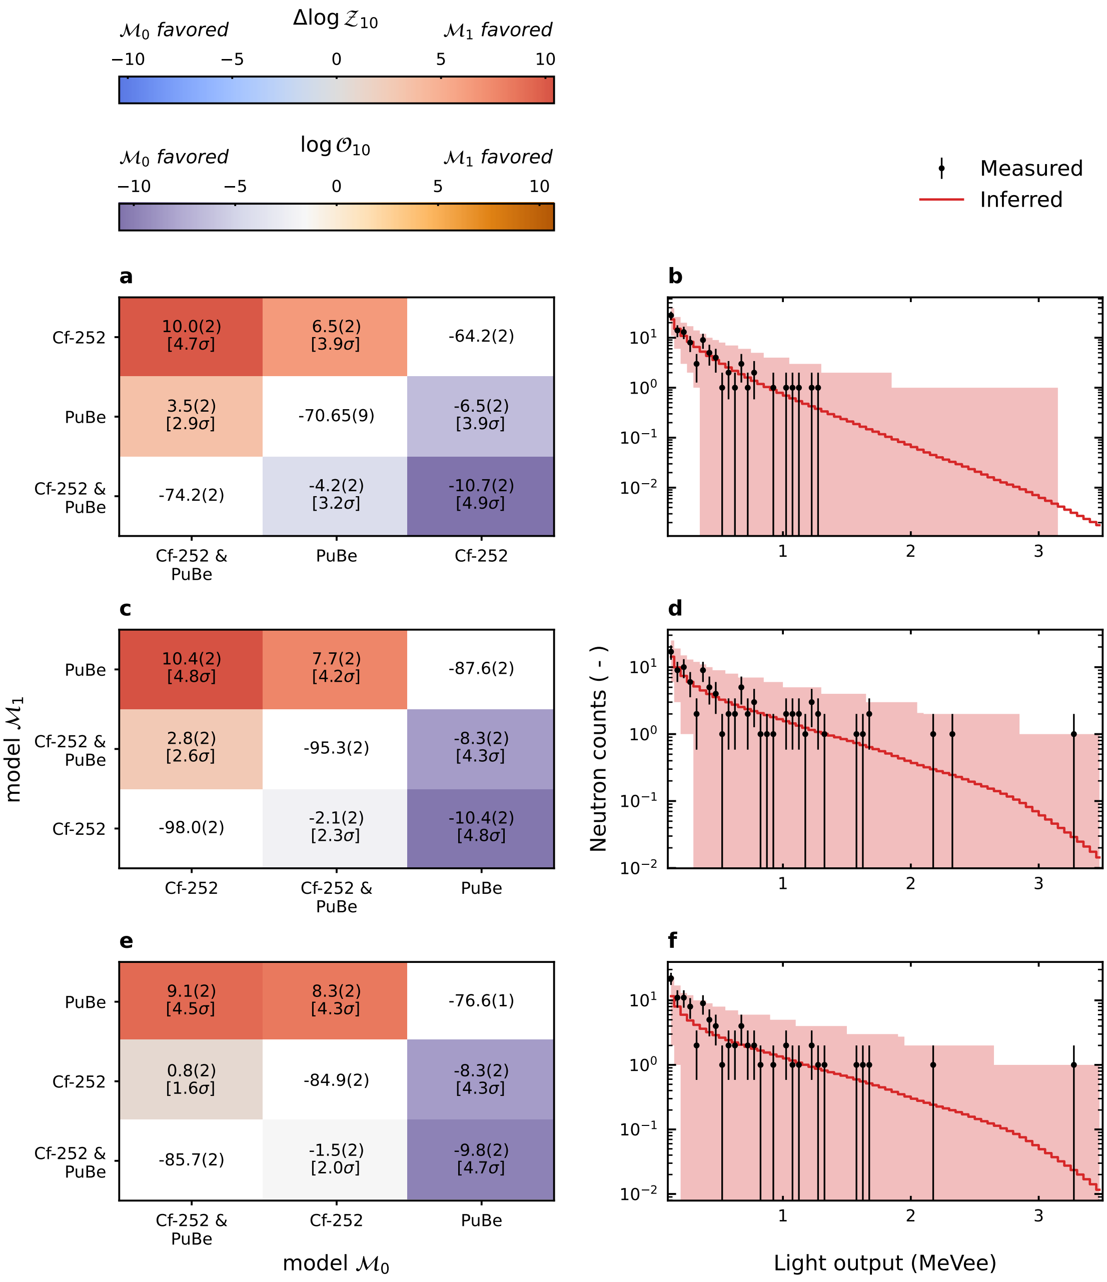


**Figure S16 Bayesian evidence results for three experiments using recoil spectroscopy with $N_{\text{event}} = 10^2$.** Same as Fig. S15, but using $N_{\text{event}} = 10^2$ events.

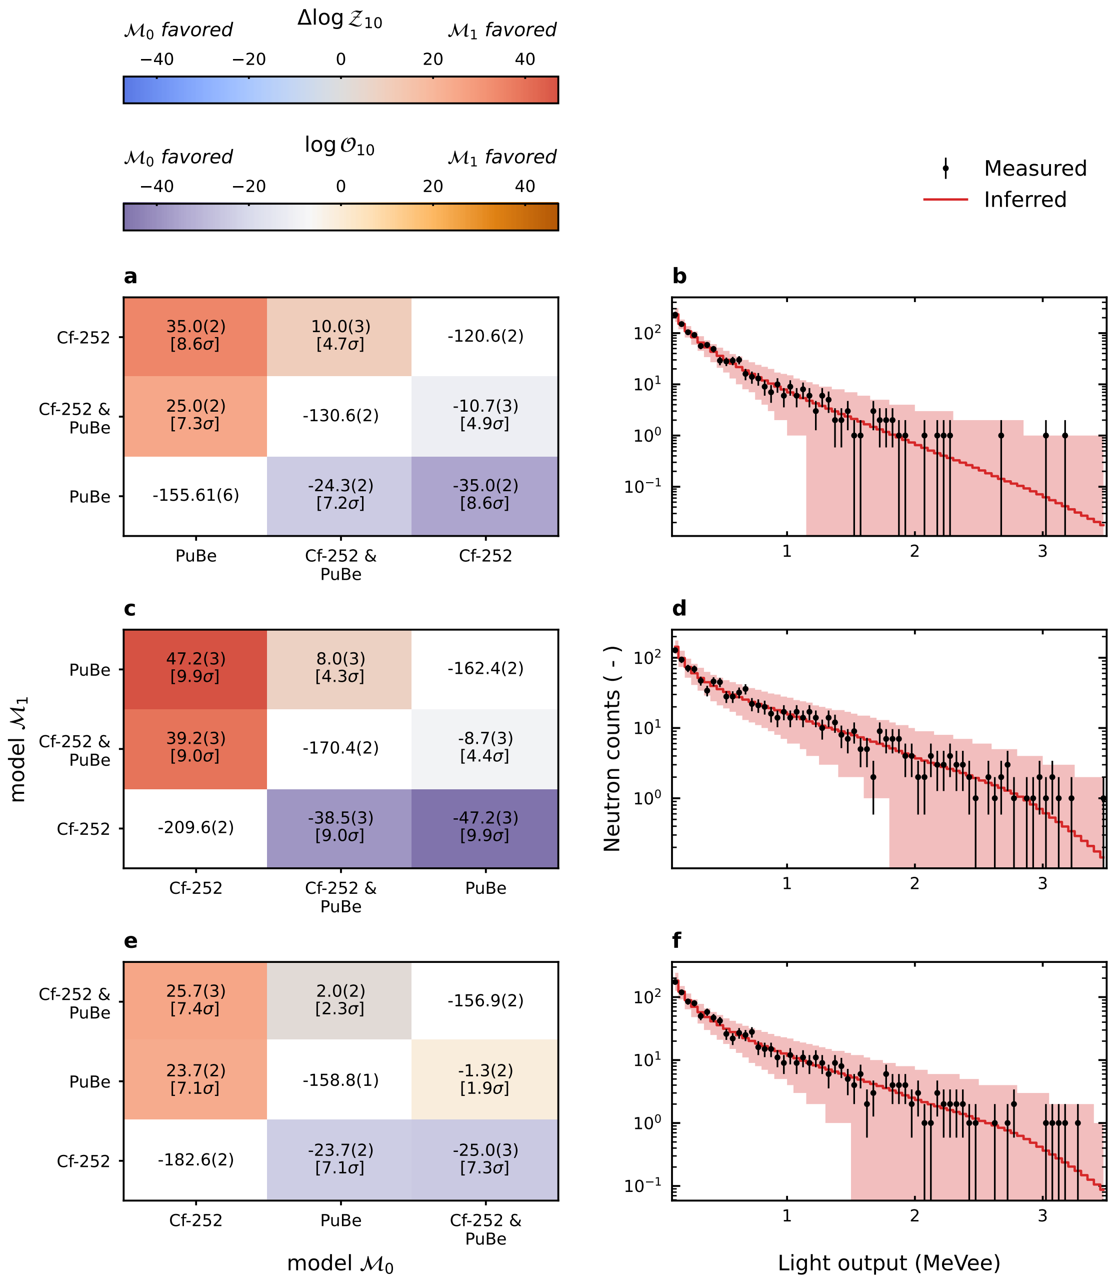


**Figure S17 Bayesian evidence results for three experiments using recoil spectroscopy with $N_{\text{event}} = 10^3$.** Same as Fig. S15, but using $N_{\text{event}} = 10^3$ events.

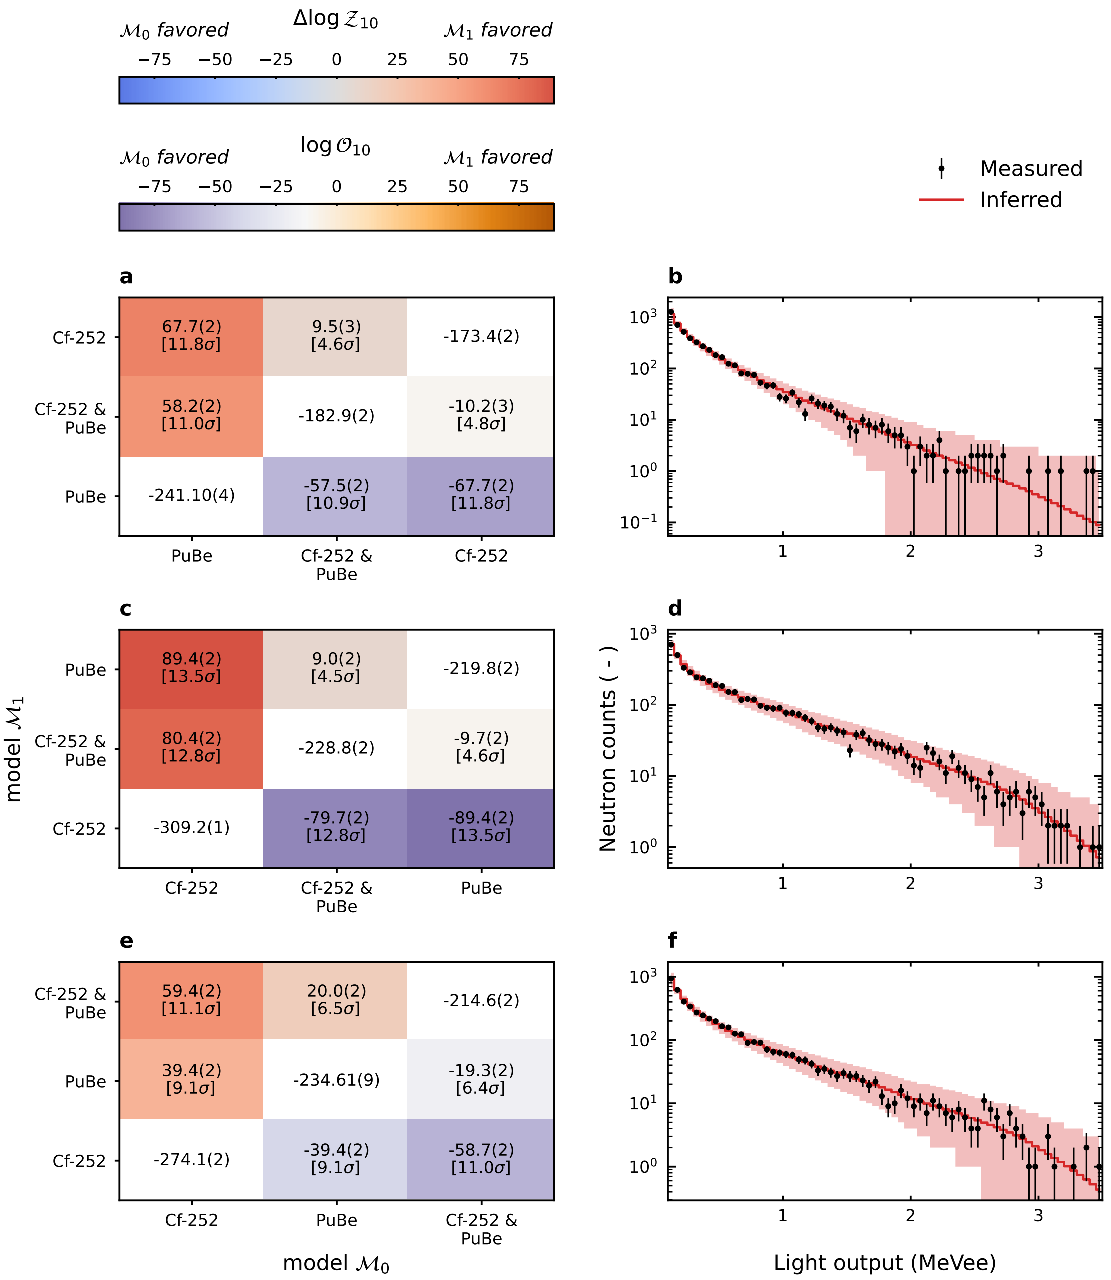


**Figure S18 Bayesian evidence results for three experiments using recoil spectroscopy with $N_{\text{event}}$ = $5 \times 10^3$.** Same as Fig. S15, but using $N_{\text{event}} = 5 \times 10^3$ events.

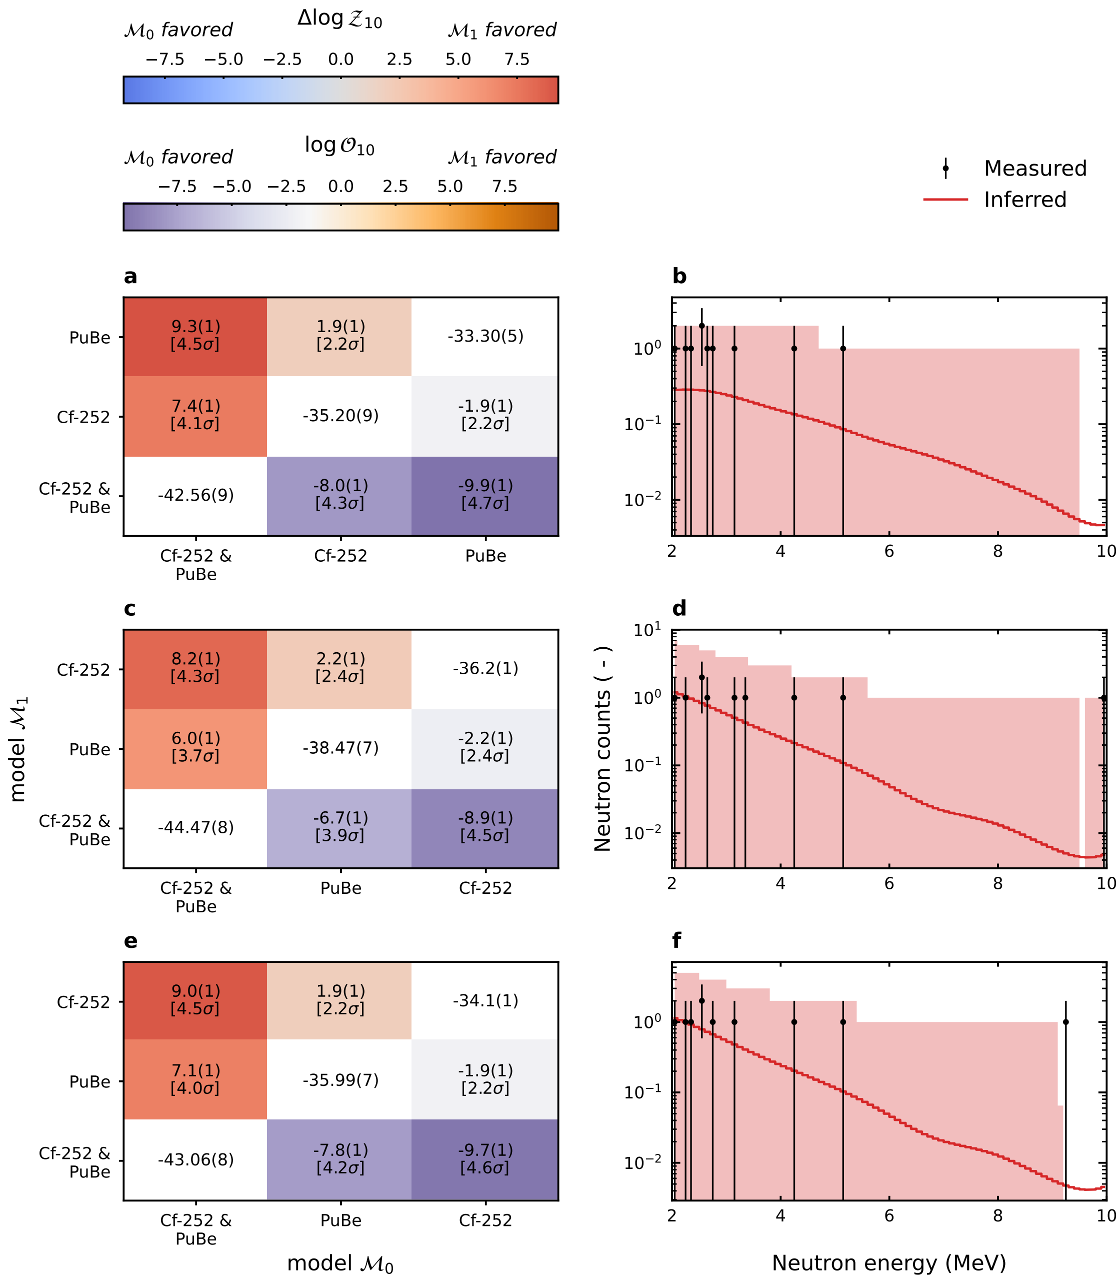


**Figure S19 Bayesian evidence results for three experiments using TOF spectroscopy with $N_{\text{event}} = 10^1$.** (a–b) Single-source Cf-252 experiment ($\mathcal{D}_1$). (c–d) Single-source PuBe experiment. (e–f) Double-source Cf-252 & PuBe experiment. Panels (a,c,e) show log evidence values $\log\mathcal{Z}_i$ for each model $\mathcal{M}_i$ (diagonal), log Bayes factors $\Delta\log\mathcal{Z}_{10} = \log\mathcal{Z}_1 - \log\mathcal{Z}_0$ (above-diagonal entries), and log posterior odds ratios $\log\mathcal{O}_{10} = \Delta\log\mathcal{Z}_{10} + \log p(\mathcal{M}_1) - \log p(\mathcal{M}_0)$ (below-diagonal entries) with $p(\mathcal{M}) \propto 4^{-\dim(\mathcal{M})}$. Uncertainties are indicated using least-significant-figure notation, with lower statistical-significance bounds in square brackets [17]. Panels (b,d,f) show the measured energy spectra (coverage factor $k = 1$) alongside maximum-a-posteriori predictions and 95 % central posterior predictive intervals (shaded area) for the retrieved (true) source set.

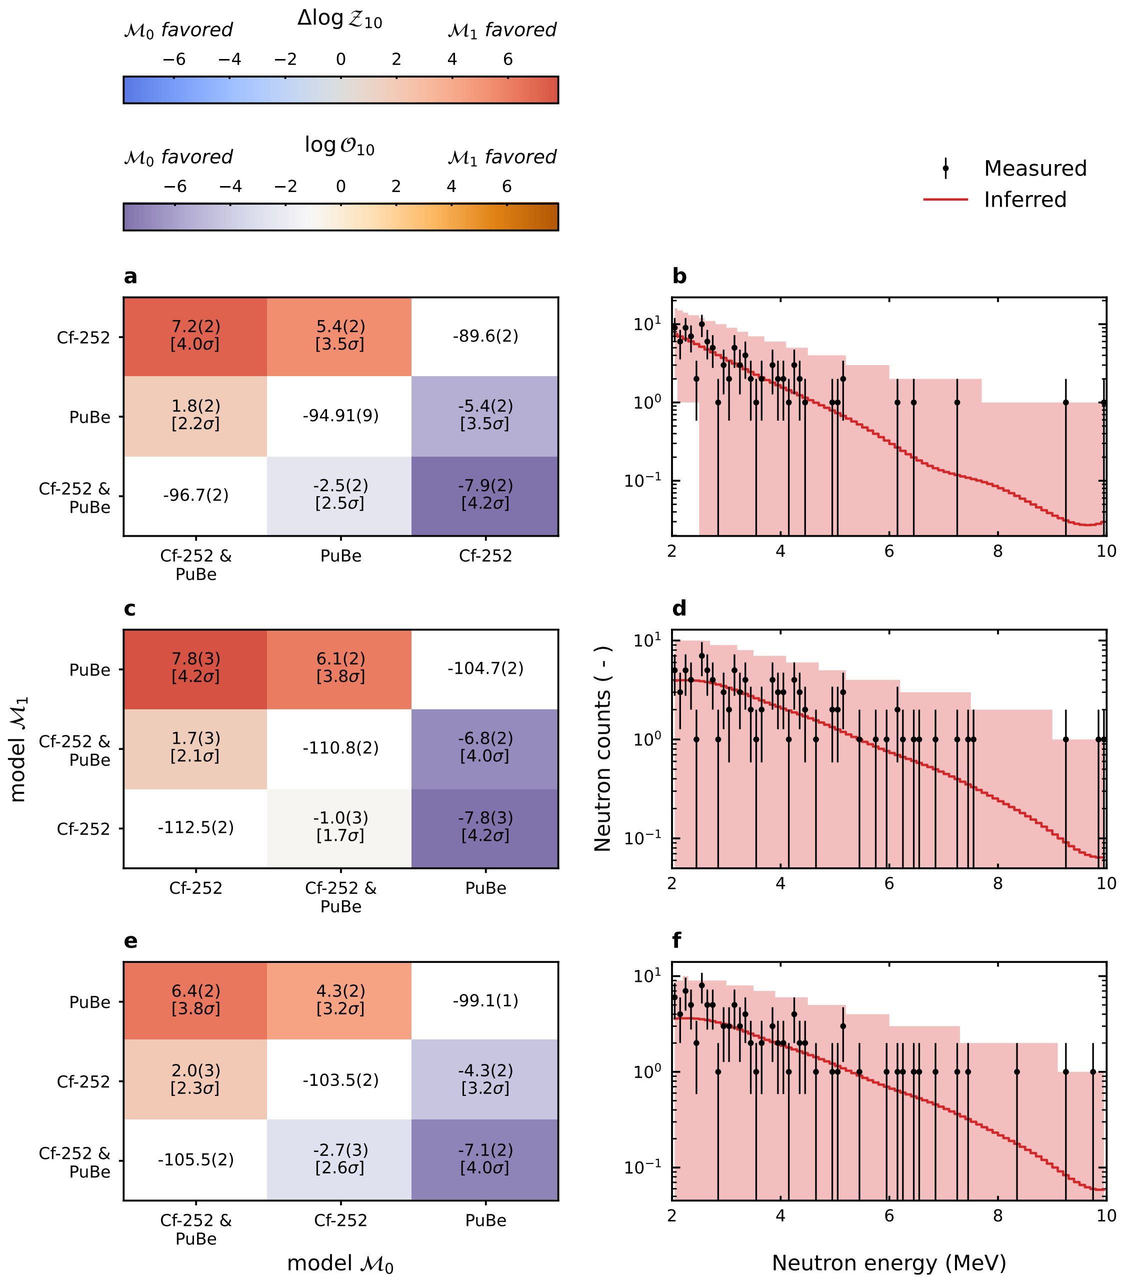


**Figure S20 Bayesian evidence results for three experiments using TOF spectroscopy with $N_{\text{event}} = 10^2$.** Same as Fig. S19, but using $N_{\text{event}} = 10^2$ events.

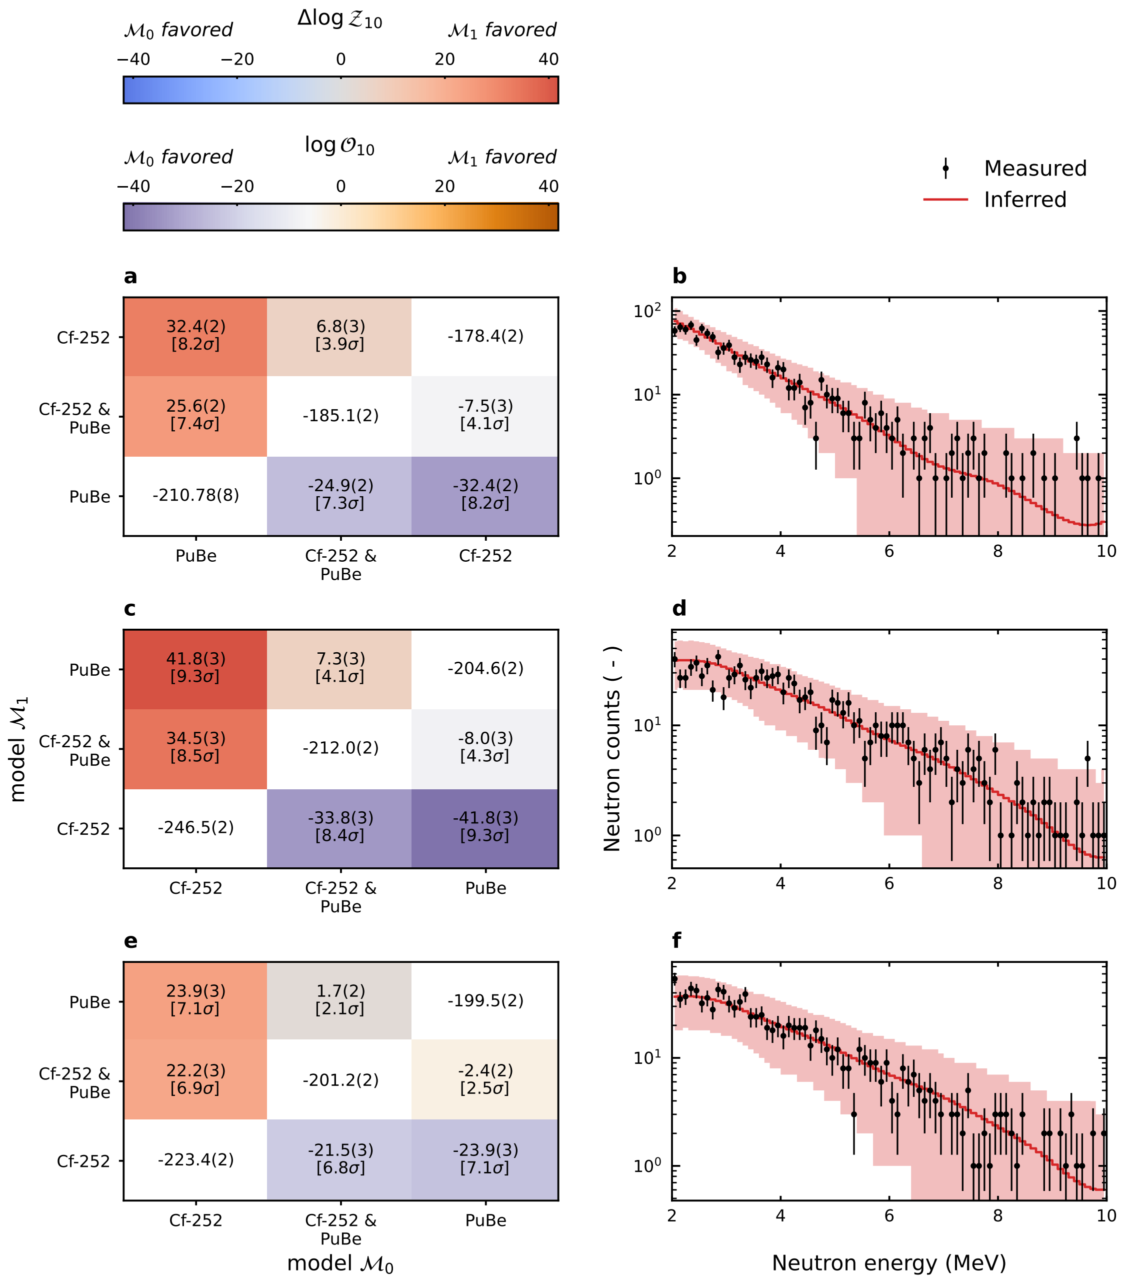


**Figure S21 Bayesian evidence results for three experiments using TOF spectroscopy with $N_{\text{event}} = 10^3$.** Same as Fig. S19, but using $N_{\text{event}} = 10^3$ events.

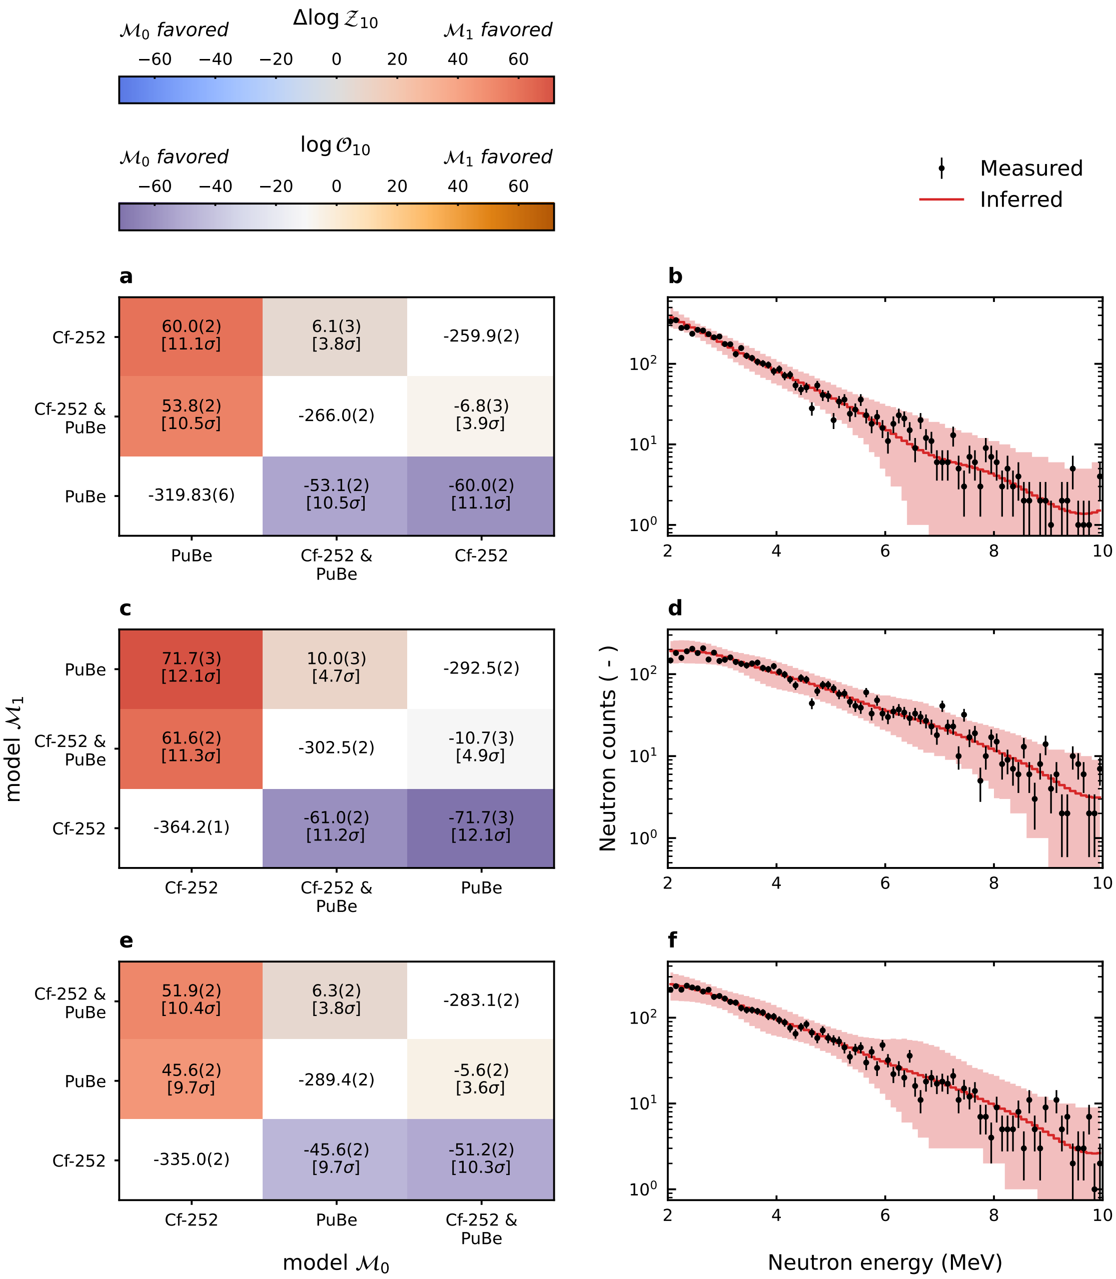


**Figure S22 Bayesian evidence results for three experiments using TOF spectroscopy with $N_{\text{event}}$ = $5 \times 10^3$.** Same as Fig. S19, but using $N_{\text{event}} = 5 \times 10^3$ events.

# Supplementary References


[1] R. Lopez, W. M. Steinberger, N. Giha, P. Marleau, S. D. Clarke, and S. A. Pozzi, Nucl. Instrum. Methods Phys. Res. A **1042**, 167407 (2022).

[2] S. D. Clarke, R. Lopez, V. Mozin, P. Kerr, J. Hutchinson, P. Marleau, and S. A. Pozzi, Sci Rep **14**, 17192 (2024).

[3] R. Lopez, O. Pakari, C. Ballard, S. Clarke, and S. Pozzi, Radiat. Meas. **184**, 107440 (2025).

[4] L. Q. Nguyen, G. Gabella, B. L. Goldblum, T. A. Laplace, J. S. Carlson, E. Brubaker, and P. L. Feng, Nucl. Instrum. Methods Phys. Res. A **988**, 164898 (2021).

[5] T. H. Shin, P. L. Feng, J. S. Carlson, S. D. Clarke, and S. A. Pozzi, Nucl. Instrum. Methods Phys. Res. A **939**, 36 (2019).

[6] W. K. Warburton, J. S. Carlson, and P. L. Feng, Nucl. Instrum. Methods Phys. Res. A **1018**, 165778 (2021).

[7] J. S. Carlson and P. L. Feng, Nucl. Instrum. Methods Phys. Res. A **832**, 152 (2016).

[8] M. L. Ruch, P. Marleau, and S. A. Pozzi, in 2016 IEEE Nucl. Sci. Symp. Med. Imaging Conf. Room-Temp. Semicond. Detect. Workshop NSSMICRTSD (Oct. 2016), pp. 1–3.

[9] N. P. Giha, W. M. Steinberger, L. Q. Nguyen, J. S. Carlson, P. L. Feng, S. D. Clarke, and S. A. Pozzi, Nucl. Instrum. Methods Phys. Res. A **1014**, 165676 (2021).

[10] N. P. Giha, M. L. Ruch, A. D. Fulvio, W. M. Steinberger, and S. A. Pozzi, in 2017 IEEE Nucl. Sci. Symp. Med. Imaging Conf. NSSMIC (Oct. 2017), pp. 1–3.

[11] W. M. Steinberger, M. L. Ruch, N. Giha, A. D. Fulvio, P. Marleau, S. D. Clarke, and S. A. Pozzi, Sci Rep **10**, 1855 (2020).

[12] W. Steinberger, N. Giha, M. Hua, S. Clarke, and S. Pozzi, Nucl. Instrum. Methods Phys. Res. A **1003**, 165266 (2021).

[13] F. D. Brooks, R. W. Pringle, and B. L. Funt, IRE Trans. Nucl. Sci. **7**, 35 (1960).

[14] J. K. Polack, M. Flaska, A. Enqvist, C. S. Sosa, C. C. Lawrence, and S. A. Pozzi, Nucl. Instrum. Methods Phys. Res. A **795**, 253 (2015).

[15] J. B. Birks, Proc. Phys. Soc. Sect. A **64**, 874 (1951).

[16] D. Servén and C. Brummitt, *pyGam: Generalized Additive Models in Python.* Zenodo, July 26, 2025.

[17] R. Trotta, Contemp. Phys. **49**, 71 (2008).

[18] M. Praszalowicz, Phys. Lett. B **704**, 566 (2011).

[19] S. V. Tezlaf, Phys. Scr. **98**, 115310 (2023).

[20] L. A. Perez, S. Malhotra, J. E. Rhoads, and V. Tilvi, ApJ **906**, 58 (2021).

[21] J. N. Fry and S. Colombi, MNRAS **433**, 581 (2013).

[22] L. Hurtado-Gil, V. J. Martínez, P. Arnalte-Mur, M.-J. Pons-Bordería, C. Pareja-Flores, and S. Paredes, A&A **601**, A40 (2017).

[23] M. Hameeda, A. Plastino, and M. C. Rocca, IOPSciNotes **2**, 015003 (2021).

[24] M. Hünnefeld et al., Proc. Sci. **395**, 1065 (2022).

[25] D. Salinas, V. Flunkert, J. Gasthaus, and T. Januschowski, Int. J. Forecast. **36**, 1181 (2020).

[26] J. O. Lloyd-Smith, PLOS ONE **2**, e180 (2007).

[27] G. Ashton et al., ApJS **241**, 27 (2019).

[28] D. E. G. Hare, J. Algorithms **25**, 221 (1997).

[29] P. Virtanen et al., Nat Methods **17**, 261 (2020).

[30] E. T. Jaynes, Phys. Rev. **106**, 620 (1957).

[31] J. S. Speagle, MNRAS **493**, 3132 (2020).

[32] E. Higson, W. Handley, M. Hobson, and A. Lasenby, MNRAS **483**, 2044 (2019).

[33] G. Ashton et al., Nat. Rev. Methods Primer 2022 21 **2**, 1 (2022).

[34] J. Skilling, Bayesian Anal. **1**, 833 (2006).

[35] E. Higson, W. Handley, M. Hobson, and A. Lasenby, Bayesian Anal. **13**, 873 (2018).

[36] D. Foreman-Mackey, J. Open Source Softw. **1**, 24 (2016).
